# Supplementary material for: Percolation Transition of K-Destinations Reveals Universal Backbone of Urban Mobility Networks
Source: arXiv:2406.15185 source file (2026-10-20)
Supplement: Supplementary file 2 [file supplementary.tex]

\documentclass[aps,pre,amsmath,amssymb,superscriptaddress]{revtex4-2}
\usepackage{rotating}
\usepackage{amsmath}
\usepackage{graphicx}
\usepackage{subcaption}
\usepackage{siunitx}
\usepackage{array}

\begin{document}

\title{Supplementary Materials for \\ Percolation transition of k-frequent destinations network for urban mobility}
\author{Weiyu Zhang}
\affiliation{Institute of Remote Sensing and Geographical Information Systems, Peking University, Yiheyuan Road 5, Haidian District, Beijing, 100871, China}
\author{Furong Jia}
\affiliation{Institute of Remote Sensing and Geographical Information Systems, Peking University, Yiheyuan Road 5, Haidian District, Beijing, 100871, China}
\author{Jianying Wang}
\affiliation{Institute of Space and Earth Information Science, The Chinese University of Hong Kong, Hong Kong}
\author{Yu Liu}
\email{liuyu@urban.pku.edu.cn}
\affiliation{Institute of Remote Sensing and Geographical Information Systems, Peking University, Yiheyuan Road 5, Haidian District, Beijing, 100871, China}
\author{Gezhi Xiu}
\affiliation{Institute of Remote Sensing and Geographical Information Systems, Peking University, Yiheyuan Road 5, Haidian District, Beijing, 100871, China}

\maketitle

\section*{Data Description}
\subsection*{Mobile Phone Data}
We utilize a comprehensive dataset detailing the intracity human mobility within the United States, spanning eight major cities from January 2018 to December 2021\cite{safegraph_patterns_2022}. This dataset records mobility patterns within the administrative boundaries at the city level, employing the Census Block Group (CBG) as the spatial unit—a statistical area used in the United States for conducting population and housing censuses. Movements are compiled into monthly Origin-Destination (OD) matrices. In each matrix, the flow from one CBG to another quantifies the total visits made by residents who lived in the origin CBG to the destination within the month. It needs to be mentioned that, despite revisions to the CBG in 2020, this dataset consistently uses the 2010-2019 version to ensure data uniformity. 

The cities included are New York, Los Angeles, Chicago, Phoenix, Philadelphia, San Diego, Dallas, and San Jose. These cities vary a lot in their size, shape, history, and socio-economic state, ranging from New York with 6,493 CBGs to San Jose with 583 CBGs. The quantity of records varies from 20 million (in San Jose) to almost 4 billion (in New York) depending on city sizes. 
This heterogeneity emphasizes the dataset's potential to delineate diverse dimensions of urban connectivity, consequently bolstering the generalizability of our study's findings.

\subsection*{Socioeconomic factors}
The socioeconomic dataset, obtained from the American Community Survey (ACS) and OpenStreetMap, utilizes CBG level information. This dataset encompasses key indicators including poverty, health insurance coverage, educational levels, the built environment, and racial segregation (Table~\ref{table:socioeconomic_indicators}), spanning from 2018 to 2021 and covers eight major U.S. cities, including New York, Los Angeles, Chicago, Houston, Phoenix, Philadelphia, San Antonio, San Diego, Dallas, and San Jose. 
% Indicators representing the number of persons were normalized by the population of CBG for further analysis.

\begin{table}[h!]
\centering
\caption{Socioeconomic Indicators}
\begin{tabular}{ll}
\hline
\textbf{Type} & \textbf{Indicator} \\
\hline
Poverty & Median Household Income \\
& The Ratio Of Income To Poverty Level Between 0.5 And 0.99 \\
& The Ratio Of Income To Poverty Level Below 0.5 \\
Health & The Ratio Of Population With No Health Insurance \\
Education & Average Population Enrolled In College \\
& Average Population That Graduated From High School \\
& Average Population With A Bachelor's Degree \\
& Average Population With A Master's Degree \\
& Average Population With A Doctorate \\
Built Environment & Building Density \\
& Driving Road Density \\
& Cycling Road Density \\
& Walking Road Density \\
& POI Density \\
& Construction Percentage \\
& Residential Percentage \\
& Racial Entropy \\
\hline
\end{tabular}
\label{table:socioeconomic_indicators}
\end{table}

\section*{Implementation details of the percolation model}
To determine the percolation threshold for each city-month pair, the process begins with setting $k=1$. We incrementally increase $k$ by one, and each time select the top $k$ outflows from each node to form a `top-k network'. This process continues until the top-k network achieves strong connectivity, meaning every node can be reached from any other node. The value of $k$ at this point is identified as the percolation threshold for the city-month pair.

In our analysis, we observed a saturation phenomenon in the percolation threshold as we progressively removed unimportant nodes that own the smallest degree in the city. Specifically, as more nodes with the lowest degrees are removed, the percolation threshold initially decreases and then stabilizes. This indicates that the least significant, peripheral areas disrupt the calculation of critical connectivity, while the core, stable urban areas' critical connectivity remains largely unaffected by the removal of additional nodes. The behavior of This core urban area is precisely what we aim to measure and depict. To illustrate this phenomenon, we present the distribution of percolation thresholds after removing the 2\%, 3\%, and 5\% of nodes with the smallest degrees in Figure~\ref{fig:distribution-k}. The results show no significant changes as more of the least connected nodes are removed, underscoring the robust structure of core urban areas. In our principal findings, we opted to exclude the bottom 2\% of nodes.

\section*{Temporal Stabilities}

\subsection*{Temporal fluctuation of connectivity at criticality}

The temporal variations of cities' critical connectivity provide additional insights into connective behaviors, supporting the argument for the consistency of the percolation threshold. We examined the percolation thresholds across 8 cities spanning 48 months, from January 2018 to December 2022. Figure~\ref{fig: k_across_time} illustrates that the overall trend of the percolation thresholds remains stable, particularly before the COVID-19 pandemic. In April 2020, the implementation of stay-at-home orders and other non-pharmaceutical interventions (NPIs) in U.S. cities significantly impacted human mobility behaviors, leading to a noticeable decline in the percolation threshold. To delve deeper into the dynamic trends, we divided our dataset into 2 phases: pre-pandemic and post-pandemic. Linear regression analyses are applied to each segment using the equation $\bar{m}=a+bt$. Our analysis revealed that pre-pandemic urban connectivity remained steady, as evidenced by the non-significant change in the mean percolation threshold over time (p = 0.64), indicating a consistent level of critical connectivity before the pandemic's onset. Interestingly, although the immediate aftermath of the pandemic onset showed a decline in connectivity, this was followed by a gradual stable rebound, as suggested by a significant slope of 1.3455 (p = 0.02) over the post-pandemic phase. This pattern underscores the inherent resilience of urban systems, which, despite experiencing initial disruptions due to pandemic-related restrictions, have begun to adapt and recover, leading to a stabilization in critical connectivity over time.

To understand the underlying mechanism of this decline and rebound behavior, it is natural to hypothesize that pandemic-induced fears and government-imposed restrictions collectively steered people towards fewer and more concentrated destinations. This behavioral shift towards more localized and limited movement patterns effectively resulted in a decrease in the city's percolation threshold. 

Additional evidence supports the hypothesis above. We introduce a metric, the effective number of destinations (END) to assess the diversity of people's movement. To compute the END, we first normalize the outflows from each CBG against its total outflows. The END is then calculated as 
$$END \equiv 1/\sum_j p\_{ij}^2$$
among which, $p\_{ij}$ represents the normalized flow from node i to node j, illustrating the proportion of flow from i to j in total outflows of node i. In scenarios of maximum diversity, where flow is evenly distributed across all destinations, the END reaches $N-1$. In contrast, when all flow concentrates on a single destination, the END is reduced to 1. Unlike the typical degree measure, the END metric assesses the distribution of flow among destinations. For instance, between two nodes with identical numbers of destinations, the one with a more even outflow distribution will have a higher END value.

We subsequently normalize the percolation thresholds against each city-month pair's average END value. The temporal trends of normalized thresholds are shown in (Figure~\ref{fig: Normalized_k_across_time}), demonstrating remarkable stability over 48 months. This stability reveals that the movement diversity can effectively explain the variation induced by the pandemic. Furthermore, the pandemic, as an unnatural event, temporarily disrupted the diversity of people's mobility, causing fluctuations in the instantaneous thresholds. %However, this also highlights the inherent stability of critical connectivity over time in the absence of such unnatural disturbances. 

%Essentially, the reduced variety and increased concentration of destinations necessitated by the pandemic conditions led to a tighter, more clustered urban connectivity network, reflecting lower thresholds for city-wide connectivity under strained circumstances.

%From January 2018 to December 2022, we examined urban connectivity across multiple cities. Figure \ref{fig: k_across_time} shows that these connections remained largely stable until the COVID-19 pandemic hit, causing a noticeable drop. We hypothesized that pandemic fears, combined with government restrictions, made people choose fewer destinations.

%We split the data into pre-pandemic and post-pandemic phases and applied a linear regression analysis using the equation $\bar{m}=a+bt$. The pre-pandemic data indicated steady urban connectivity (p = 0.3). However, post-pandemic data revealed an increase, with a significant slope of 1.3455 (p = 0.02).

%This suggests that while urban connectivity was stable before the pandemic, there was a decline during the pandemic, followed by a recovery. This change in connectivity, represented by $k^*$, may indicate that people limited their destinations during the pandemic, but began to diversify them as restrictions eased. This resilience in urban connectivity is a testament to cities' adaptability during crises.
\subsection*{Power Law exponents}
Given the power-law in-degree distribution observed in the backbone extracted using the percolation threshold, variations in power-law exponents furnish extensive insights for cross-city comparisons and temporal dynamics. Comprehensively displaying the power-law exponents of in-degree distribution across cities and over time in Figure~\ref{fig:powerlaw_exponents}, two obvious trends can be recognized. Comparing exponents across cities reveals that the absolute value of the exponent, commonly referred to as alpha, tends to positively correlate with the city scale. A larger alpha value signifies a faster decay rate in the power-law distribution, indicating that larger cities tend to have a more pronounced hierarchical structure. Specifically, this suggests that in larger cities, connectivity is concentrated among fewer, highly connected nodes (such as major hubs or central areas), while in small cities the distribution of connectivity is more uniform. This observation is consistent with previous research on scale-free networks, which suggests that as cities expand, their alpha value tends to rise, surpassing 2~\cite{del2011all}. 

Besides, observing the alphas horizontally, the temporal trend of the power law exponents can correspond to the trends of k and supports our hypothesis of people's movement behavior shift. At the onset of the pandemic in April 2020, a significant transition was observed in the power law exponents across all cities, and the alphas after the pandemic are generally higher than before. On one hand, the change in the alphas reflects the impact of the pandemic on urban structures, manifested in how locations are interconnected with each other. On the other hand, the observed increase in the power-law exponent indicates a decrease in the number of core urban areas, aligning with our previously discussed hypotheses that the pandemic has led people to gravitate toward fewer and more concentrated destinations.

\section*{Spatial distribution of the Proportion of Principal Destinations}

\subsection*{Los Angeles}

Figure~\ref{fig:la_ppd} demonstrates the spatial distribution of the Proportion of Principal Destinations (PPD) across Los Angeles, revealing distinct patterns of urban engagement and socioeconomic status. High PPD values are predominantly associated with affluent neighborhoods, such as Los Feliz, a celebrity-filled enclave adjacent to Hollywood. This proximity to the urban hub of activity reflects its high accessibility and convenience, facilitating easy access to daily services and fulfilling the needs of its residents. Conversely, regions marked by lower PPD values denote communities of medium to low income, frequently tarnished by crime and insecurity. In particular, neighborhoods around the University of Southern California are notorious for elevated security risks, including widespread gang presence. Areas such as Jefferson Park and Mid City serve as prime examples where diminished PPD values align with socioeconomic challenges and safety issues, adversely affecting their overall habitability and security. In conclusion, the contrast between the high PPD values in Los Angeles' affluent neighborhoods and the lower PPD values in areas fraught with challenges underscores the diverse socioeconomic landscape across the city.

\subsection*{Philadelphia}

Figure~\ref{fig:philadelphia_ppd} demonstrates the spatial distribution of PPD values within Philadelphia. It is observed that areas with low PPD values are predominantly concentrated in the Northeast and Northern Philadelphia. In certain regions with low PPD values, a pattern emerges showing proximity to suburban expanses, parks, and rivers, often characteristic of near-suburban residential zones. In addition, areas characterized by low PPD values are commonly associated with poor neighborhoods. One such area is the Lawncrest neighborhood of Philadelphia, which has seen a staggering 291\% increase in impoverished residents from 1990 to 2017, indicative of the regional decline. High crime rates often accompany economic hardship in areas like Frankford, which is also marked by a low median household income. Similarly, neighborhoods such as Strawberry Mansion and Hunting Park, situated in the north, are recognized as dangerous zones within Philadelphia, historically infamous for their adverse conditions. Those regions identified by low PPD values, frequently beset with socioeconomic challenges, underscore the intertwined issues of safety and poverty.

\section*{Relationship between socioeconomic factors and PPD}
\subsection*{Correlation of socioeconomic factors with PPD}
In Fig. 4B, we illustrate the correlation coefficients between seventeen socioeconomic factors and the PPD values across eight cities. Table~\ref{table:ny} details the results of the correlation analysis and linear regression of these factors with PPD in New York for June 2018.

\begin{table}[h!]
\centering
\caption{Correlation analysis and linear regression of socioeconomic factors with the Proportion of Principal Destinations (PPD) in New York, June 2018.}
\begin{tabular}{lS[table-format=1.2]S[table-format=1.2]S[table-format=1.2]S[table-format=1.2]S[table-format=1.2]}
% \begin{tabular}{llllll}
\hline
\textbf{Socioeconomic Factor}                                           & \textbf{Slope}      & \textbf{Intercept} & {$\mathbf{R}^{\textbf{2}}$}        & \textbf{$\mathbf{p}$-value}   & \textbf{Correlation Coefficient} \\
\hline
Median Household Income                                 & 0.05    & 0.95 & 0.06  & {$<1\mathrm{e}-3$}  & 0.25       \\
The Ratio Of Income To Poverty Level Between 0.5 And 0.99 & -0.04 & 0.99 & 0.04 &   {$<1\mathrm{e}-3$}  & -0.21     \\
The Ratio Of Income To Poverty Level Below 0.5            & -0.04   & 0.99 & 0.04  &  {$<1\mathrm{e}-3$}  & -0.20    \\
The Ratio of No Health Insurance   & -0.03 & 0.98  & 0.02 &   {$<1\mathrm{e}-3$}  & -0.16     \\
Average Population Enrolled In College                  & -0.02 & 0.98 & 0.02 &  {$<1\mathrm{e}-3$}  & -0.13     \\
Average Population That Graduated From High School      & -0.02  & 0.98 & 0.02  &  {$<1\mathrm{e}-3$} & -0.13    \\
Average Population With A Bachelor's Degree             & 0.03  & 0.95 & 0.03 &   {$<1\mathrm{e}-3$} & 0.16      \\
Average Population With A Master's Degree               & 0.04   & 0.95 & 0.04  &  {$<1\mathrm{e}-3$}   & 0.20      \\
Average Population With A Doctorate                     & 0.02  & 0.96 & 0.01 &   {$<1\mathrm{e}-3$}  & 0.12       \\
Building Density                                        & 0.02  & 0.96 & 0.01 &   {$<1\mathrm{e}-3$}  & 0.12       \\
Driving Road Density                                    & 0.02  & 0.96 & 0.02 &   {$<1\mathrm{e}-3$}  & 0.13      \\
Cycling Road Density                                    & 0.03  & 0.96 & 0.02  &   {$<1\mathrm{e}-3$}  & 0.14       \\
Walking Road Density                                    & 0.02  & 0.96 & 0.02 &   {$<1\mathrm{e}-3$}  & 0.12       \\
POI Density                                             & 0.01  & 0.96 & 0.00 &   {$<1\mathrm{e}-3$}  & 0.05       \\
Construction Percentage  & -0.04  & 0.99 & 0.00 &   {$<1\mathrm{e}-3$}  & -0.06    \\
Residential Percentage  & -0.02 & 0.98 & 0.00 &  {$<1\mathrm{e}-3$}   & -0.06    \\
Racial Entropy & -0.01 & 0.98 & 0.00 &   {$<1\mathrm{e}-3$} & -0.07     \\
\hline
\end{tabular}
\label{table:ny}
\end{table}

\subsection*{Shift of the significance around the critical connectivity threshold}

Figure~\ref{fig:significance} displays the relationships between the number of principal destinations and the $p$-values of regressions linking socioeconomic factors with the PPD across seven cities, complementing Fig. 4A in the main text. In cities like Chicago and Philadelphia, there is a sharp increase in the significance level of socioeconomic factors, such as racial entropy and driving road density, as the $k$-most-frequent-destination subnetworks evolve from fragmented components to city-wide connectivity at the percolation threshold. While for subnetworks with the number of primary destinations more than the critical connectivity threshold, $k^*$, a noticeable drop and continuous fluctuations in the significance level for many factors are observed. In cities such as Chicago and San Jose, immediate increases in $p$-values of a few factors, such as the average population with a doctorate, are evident. The shift of significance level implies that there is an optimal level of connectivity, represented by the percolation threshold, which maximizes the influence of the socioeconomic factors on the urban network’s structure.

\begin{figure}
    \centering
    \begin{subfigure}[b]{0.6\textwidth}
        \includegraphics[width=\textwidth]{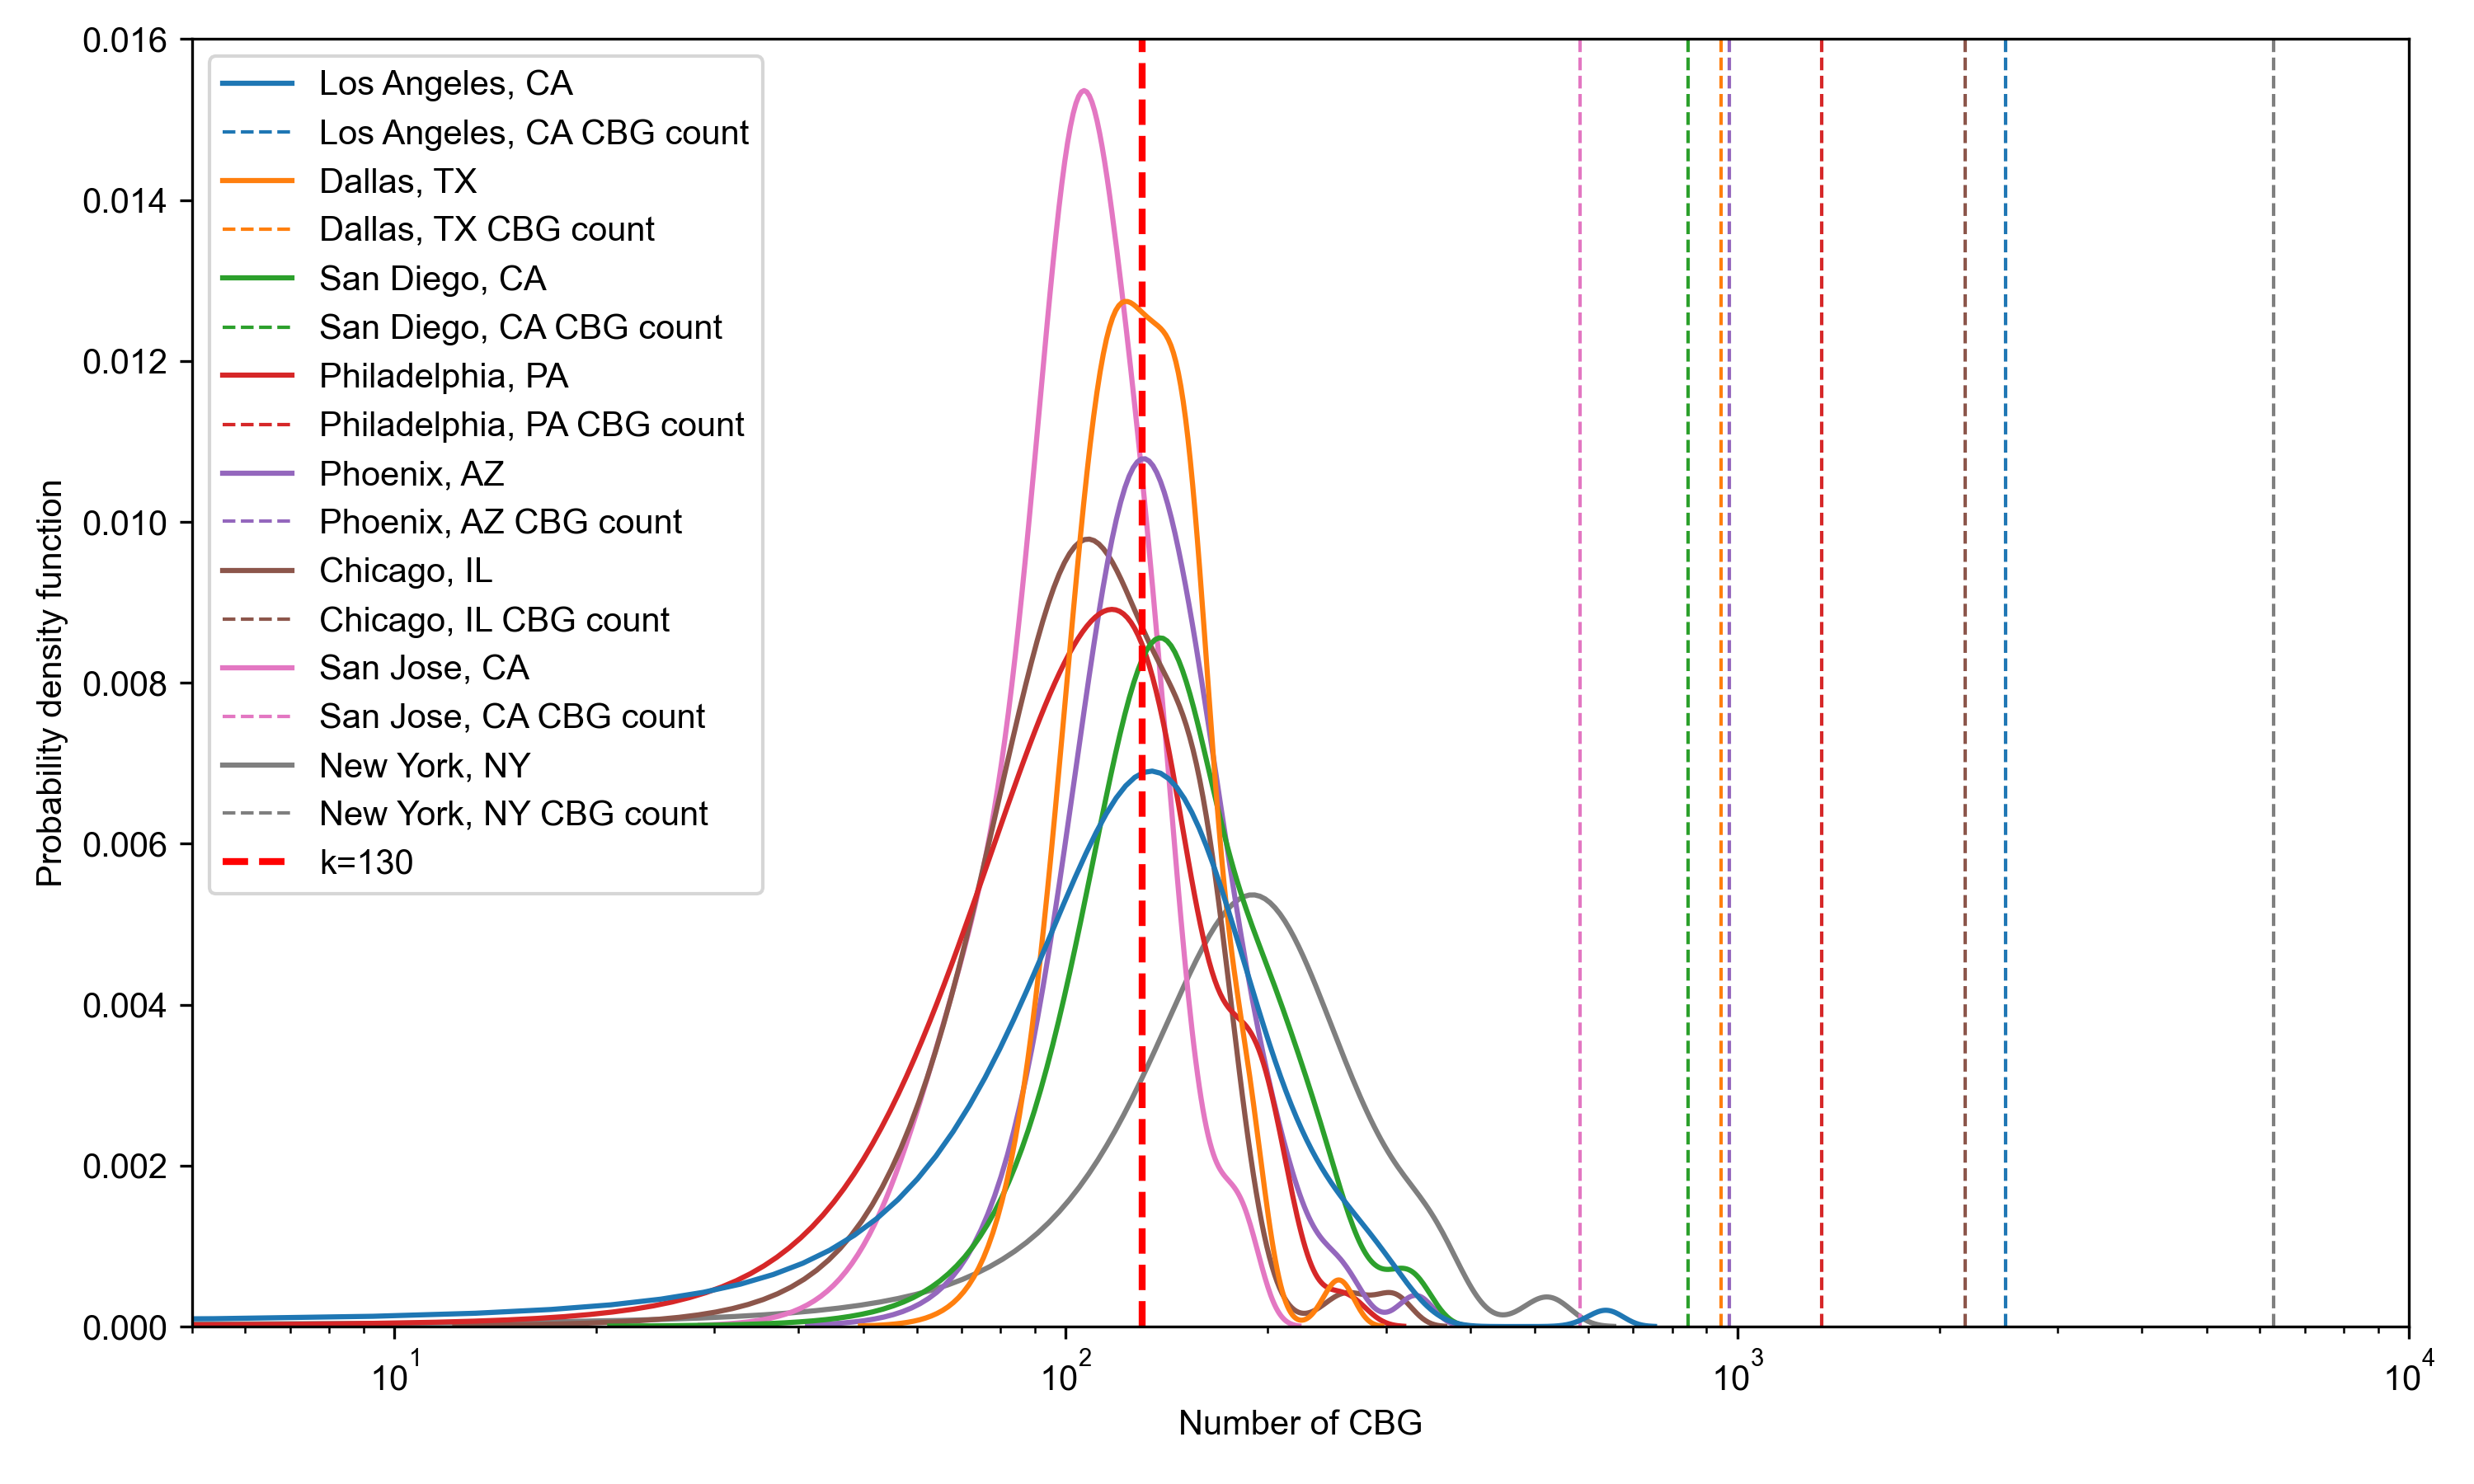}
        \caption{The distribution of percolation thresholds after removing the 2\% of nodes with the smallest degrees.}
        \label{fig:sub1}
    \end{subfigure}
    
    \begin{subfigure}[b]{0.6\textwidth}
        \includegraphics[width=\textwidth]{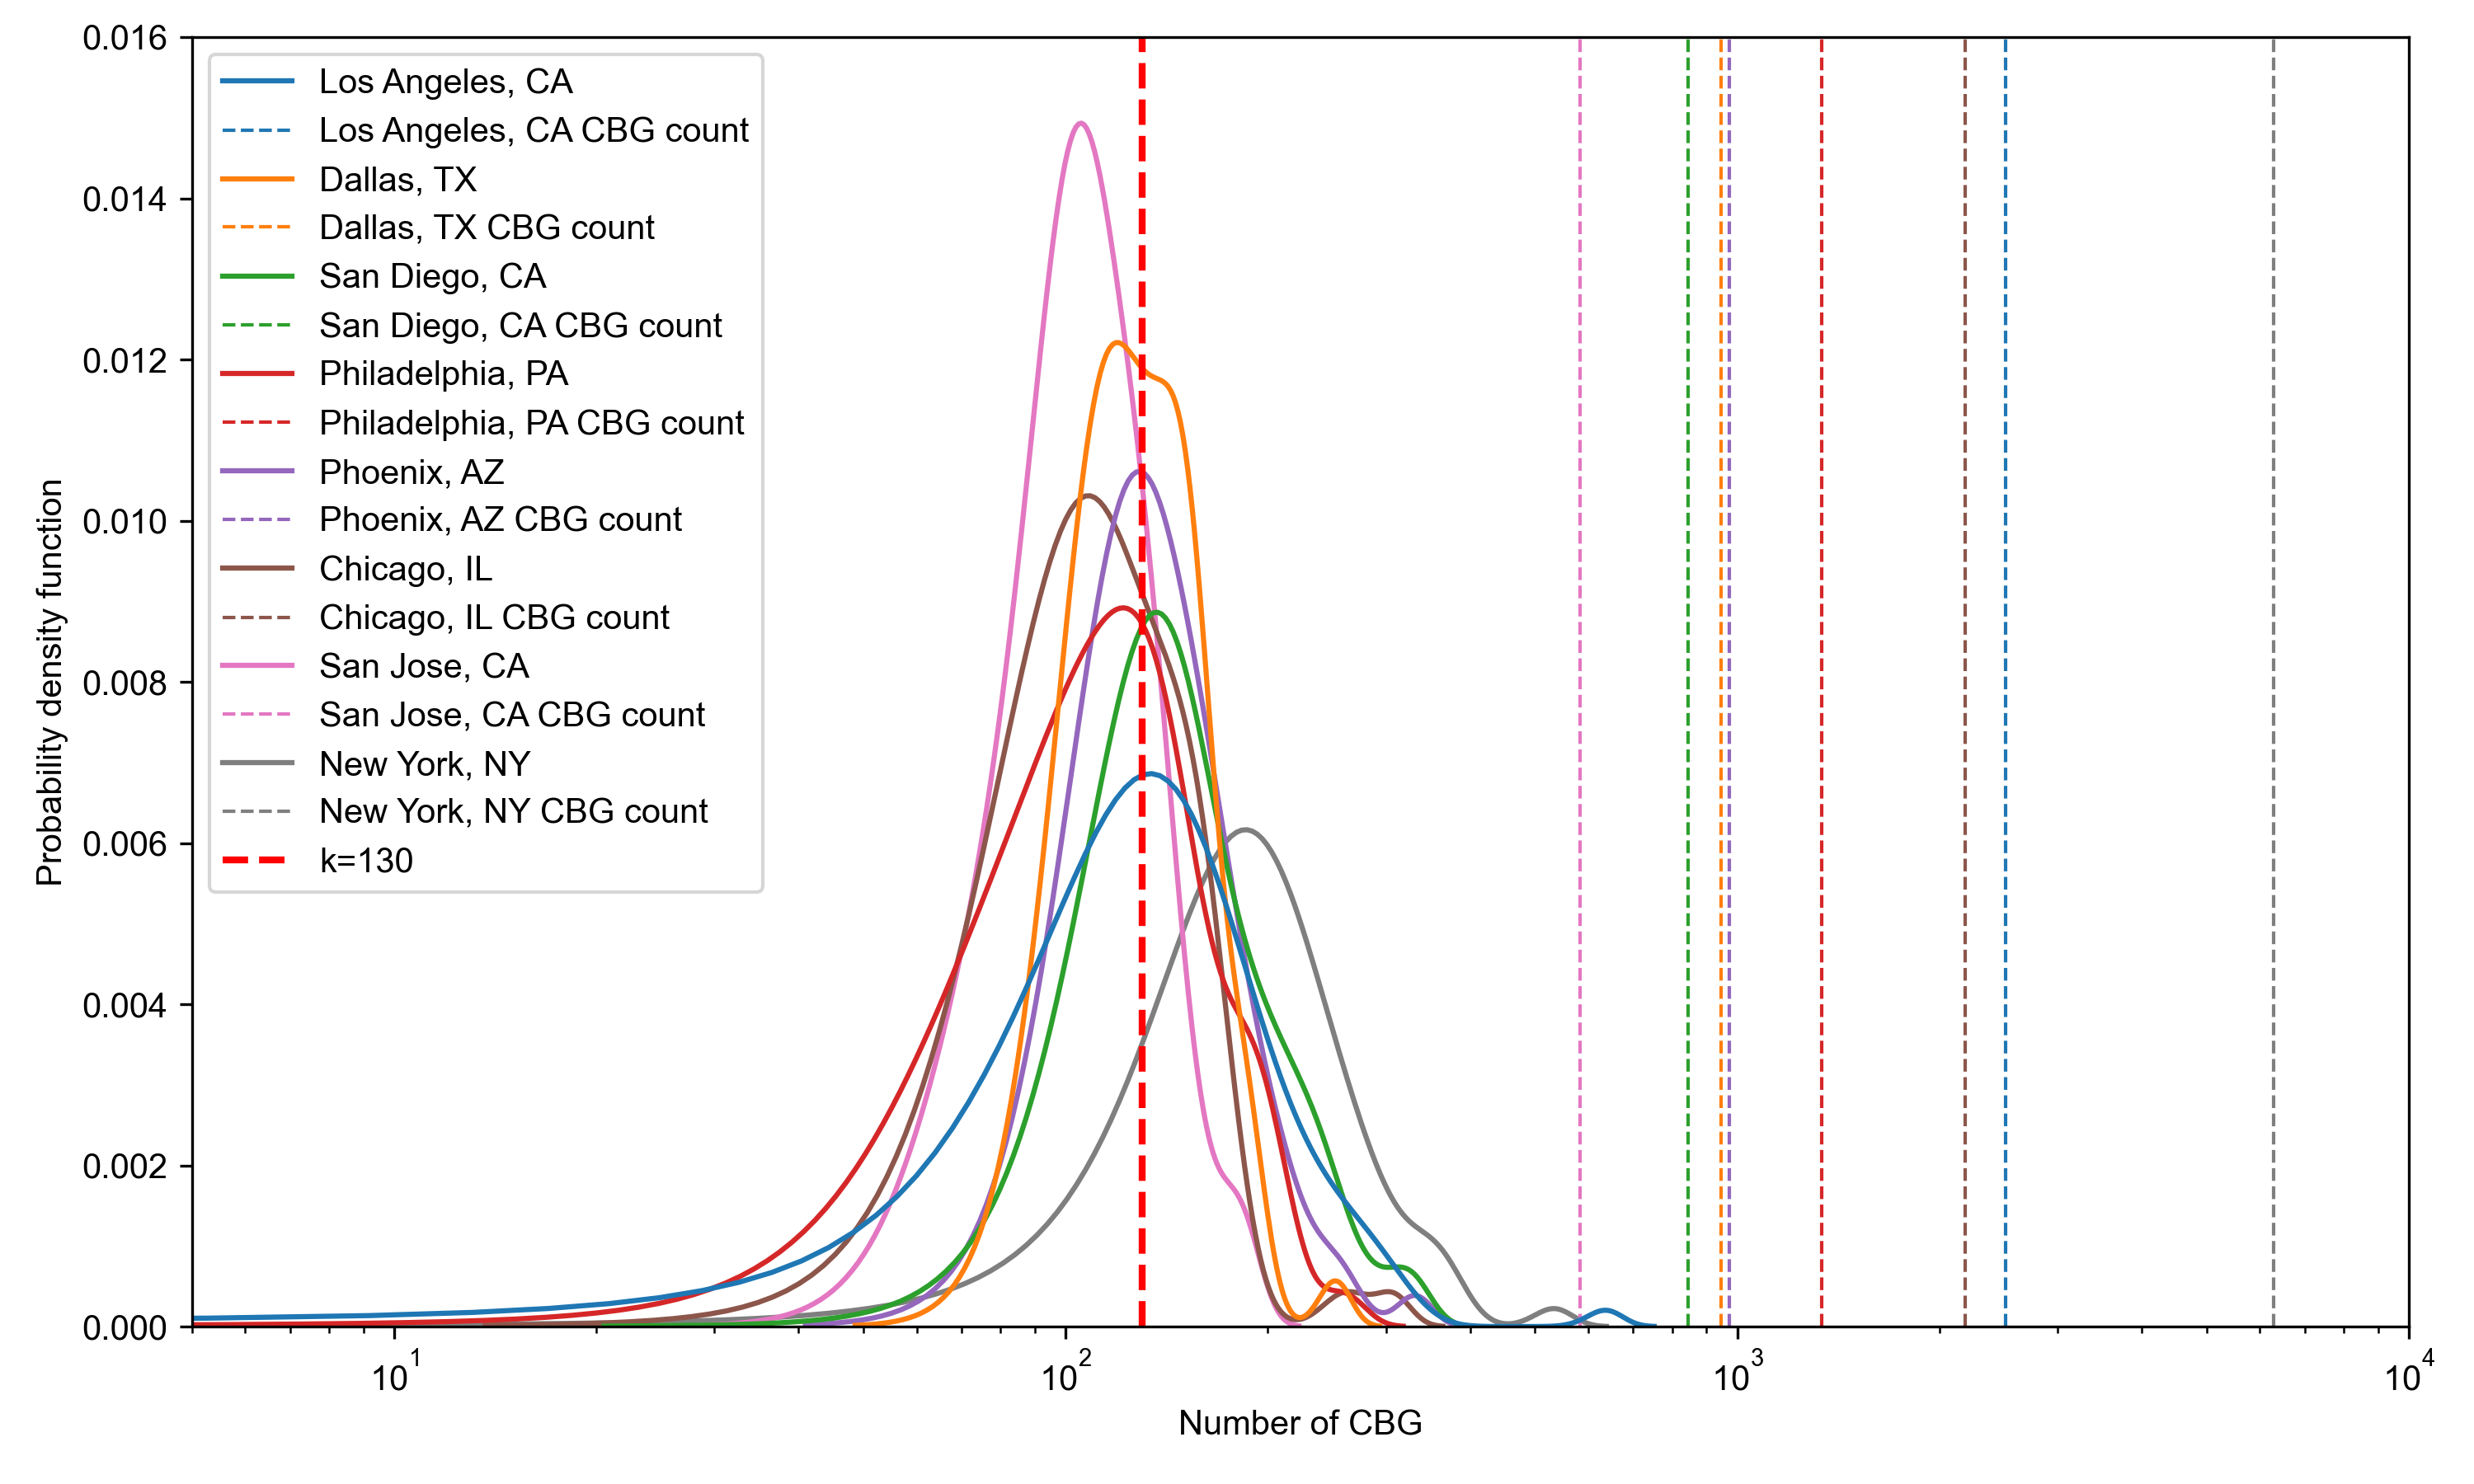}
        \caption{The distribution of percolation thresholds after removing the 3\% of nodes with the smallest degrees.}
        \label{fig:sub2}
    \end{subfigure}
    
    \begin{subfigure}[b]{0.6\textwidth}
        \includegraphics[width=\textwidth]{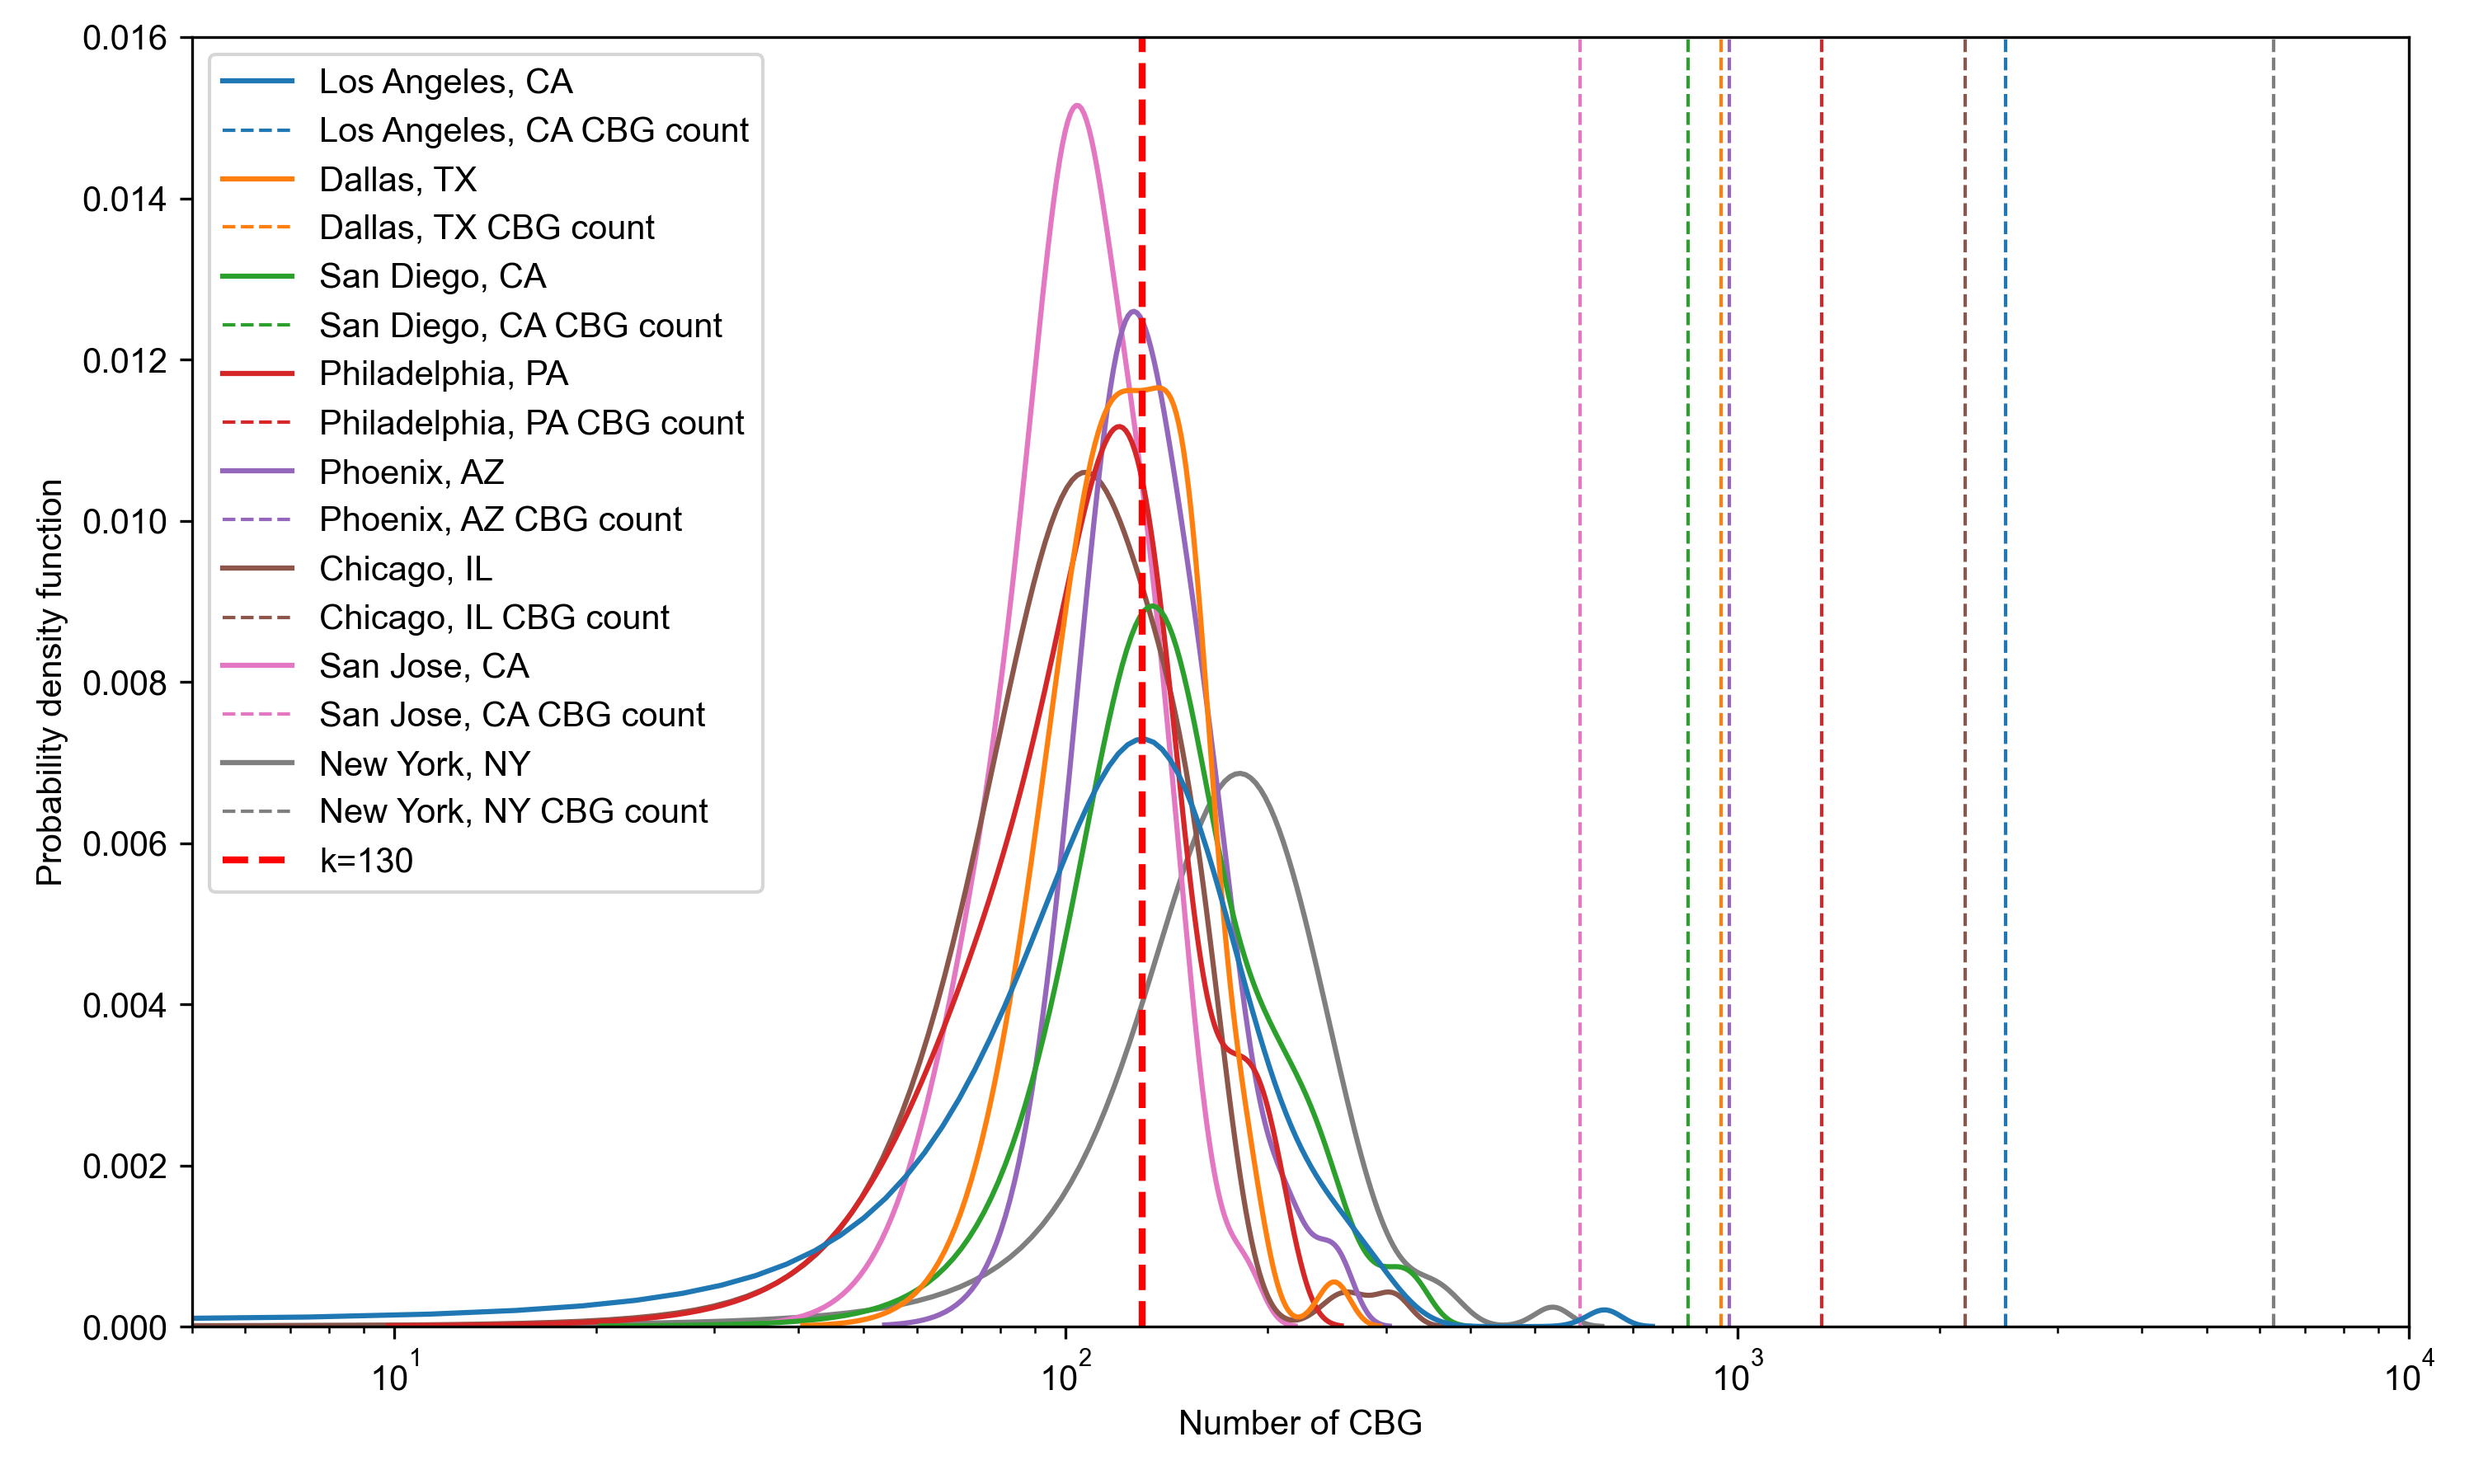}
        \caption{The distribution of percolation thresholds after removing the 5\% of nodes with the smallest degrees.}
        \label{fig:sub3}
    \end{subfigure}
    
    \caption{The Distribution of percolation thresholds in different cities under three preprocessing conditions: removal of (a) 2\%, (b) 3\%, and (c) 5\% of nodes with the smallest degrees. }
    \label{fig:distribution-k}
\end{figure}

\begin{figure}
    \centering
    \begin{subfigure}{\linewidth}
        \centering
        \includegraphics[width=\linewidth]{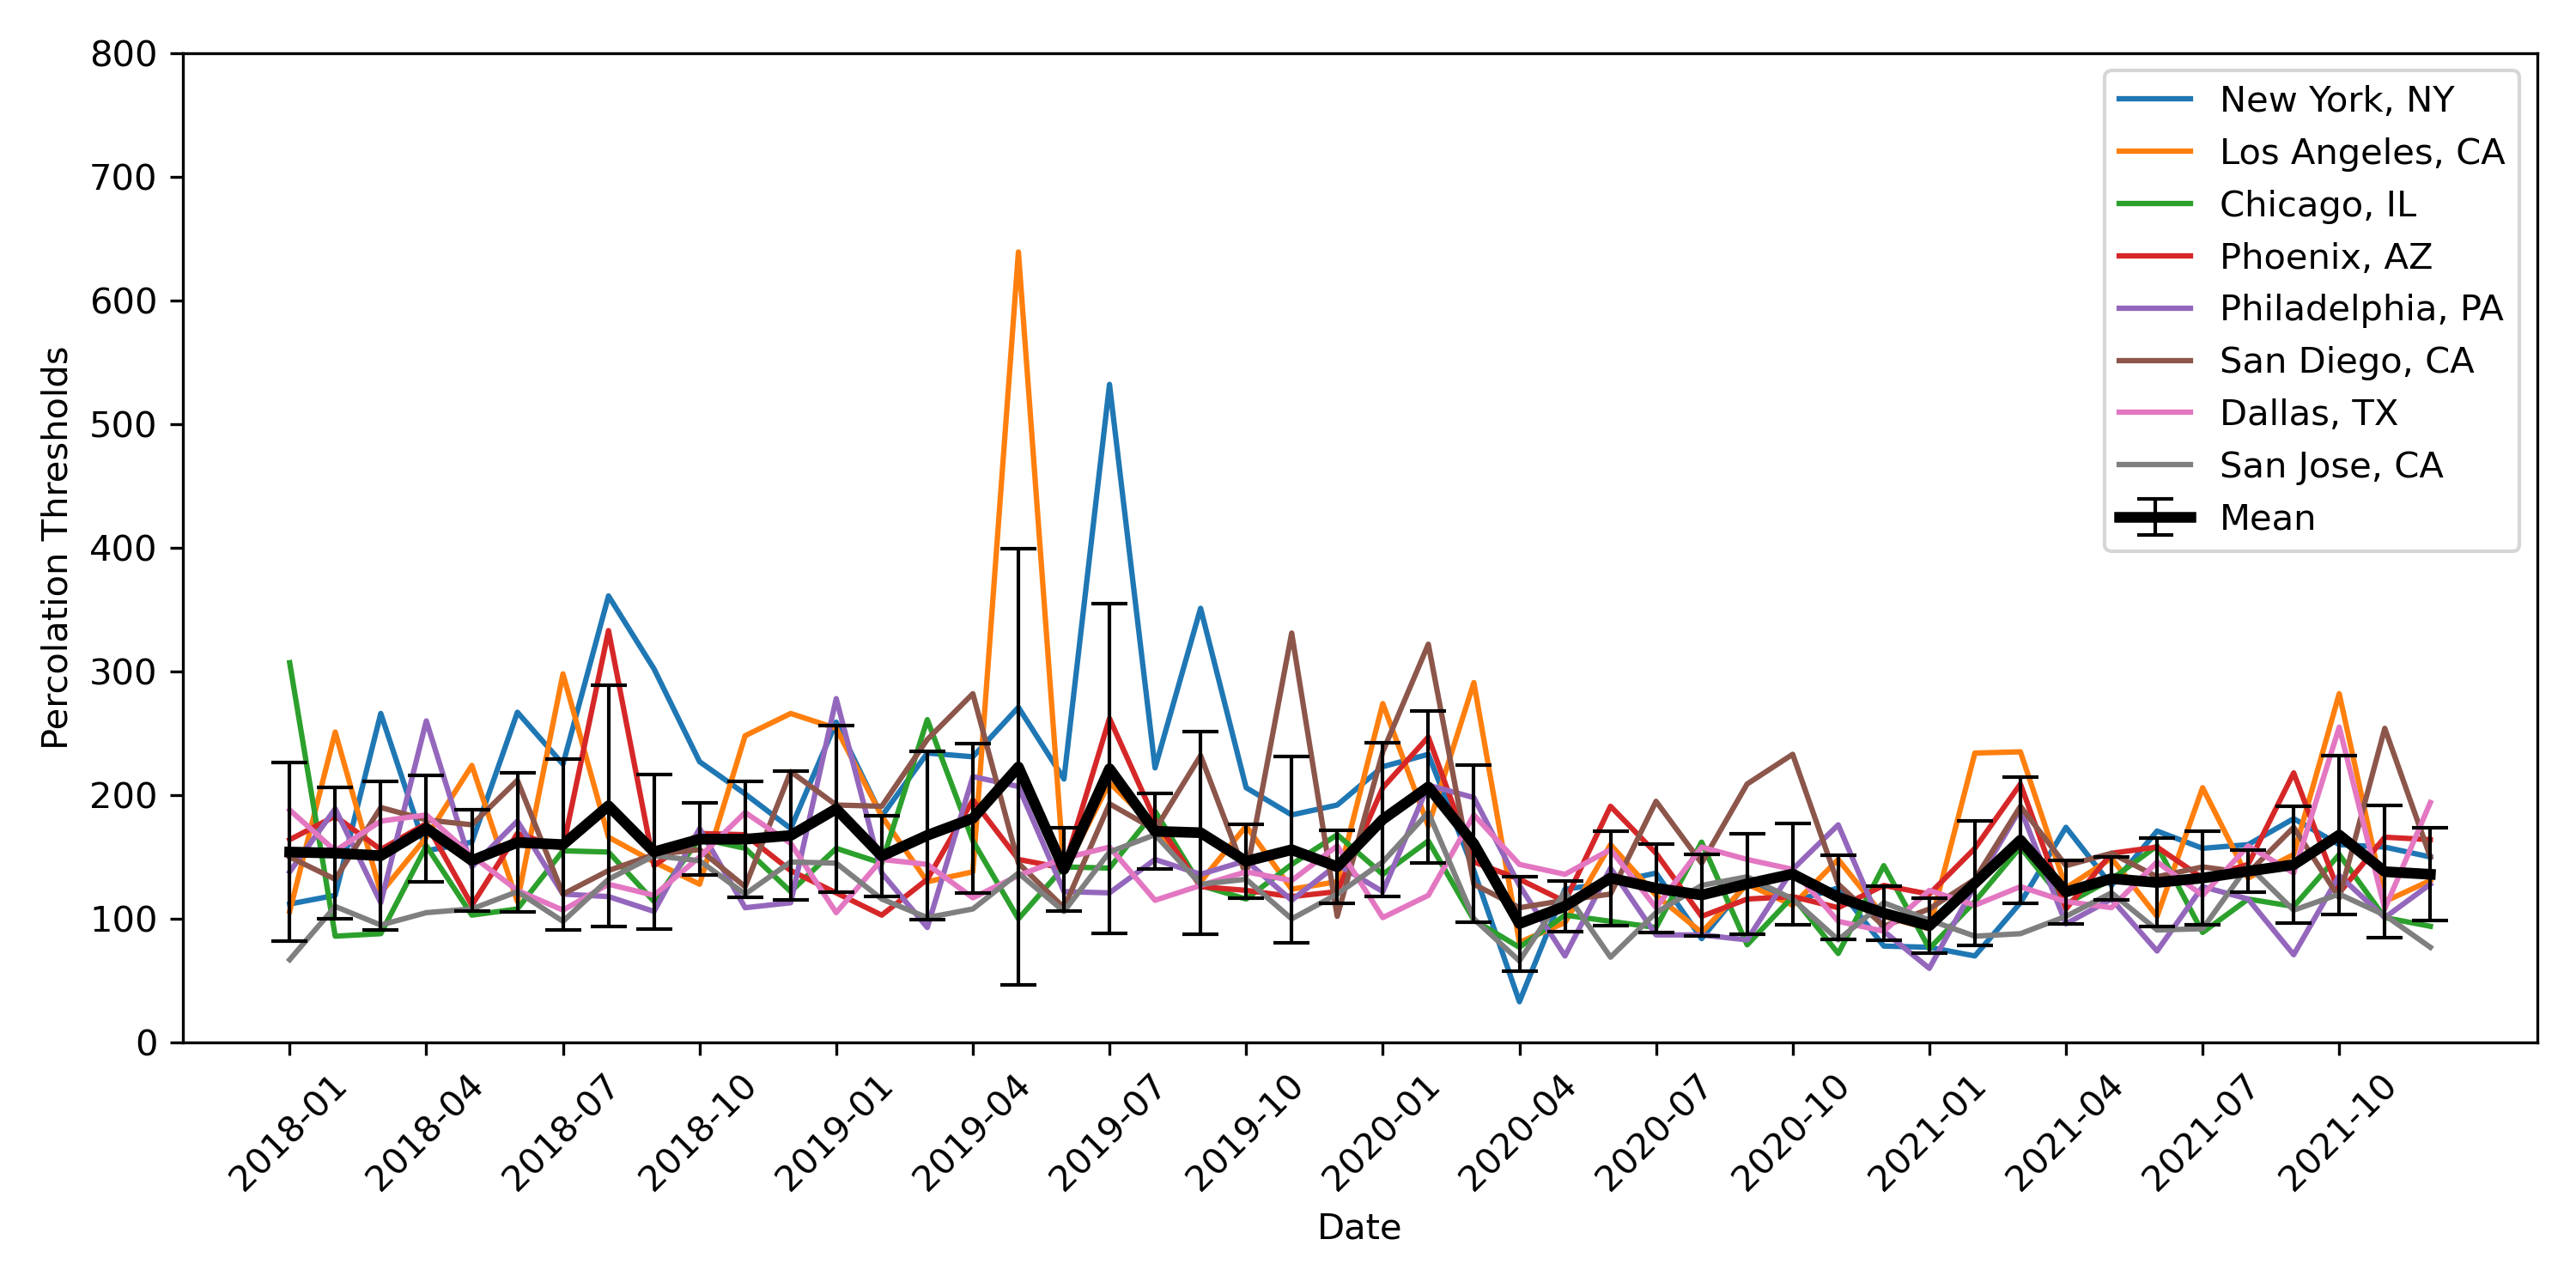}
        \caption{Variation in percolation thresholds for each city over a 48-month period.}
        \label{fig: k_across_time}
    \end{subfigure}
    \vfill
    \begin{subfigure}{\linewidth}
        \centering
        \includegraphics[width=\linewidth]{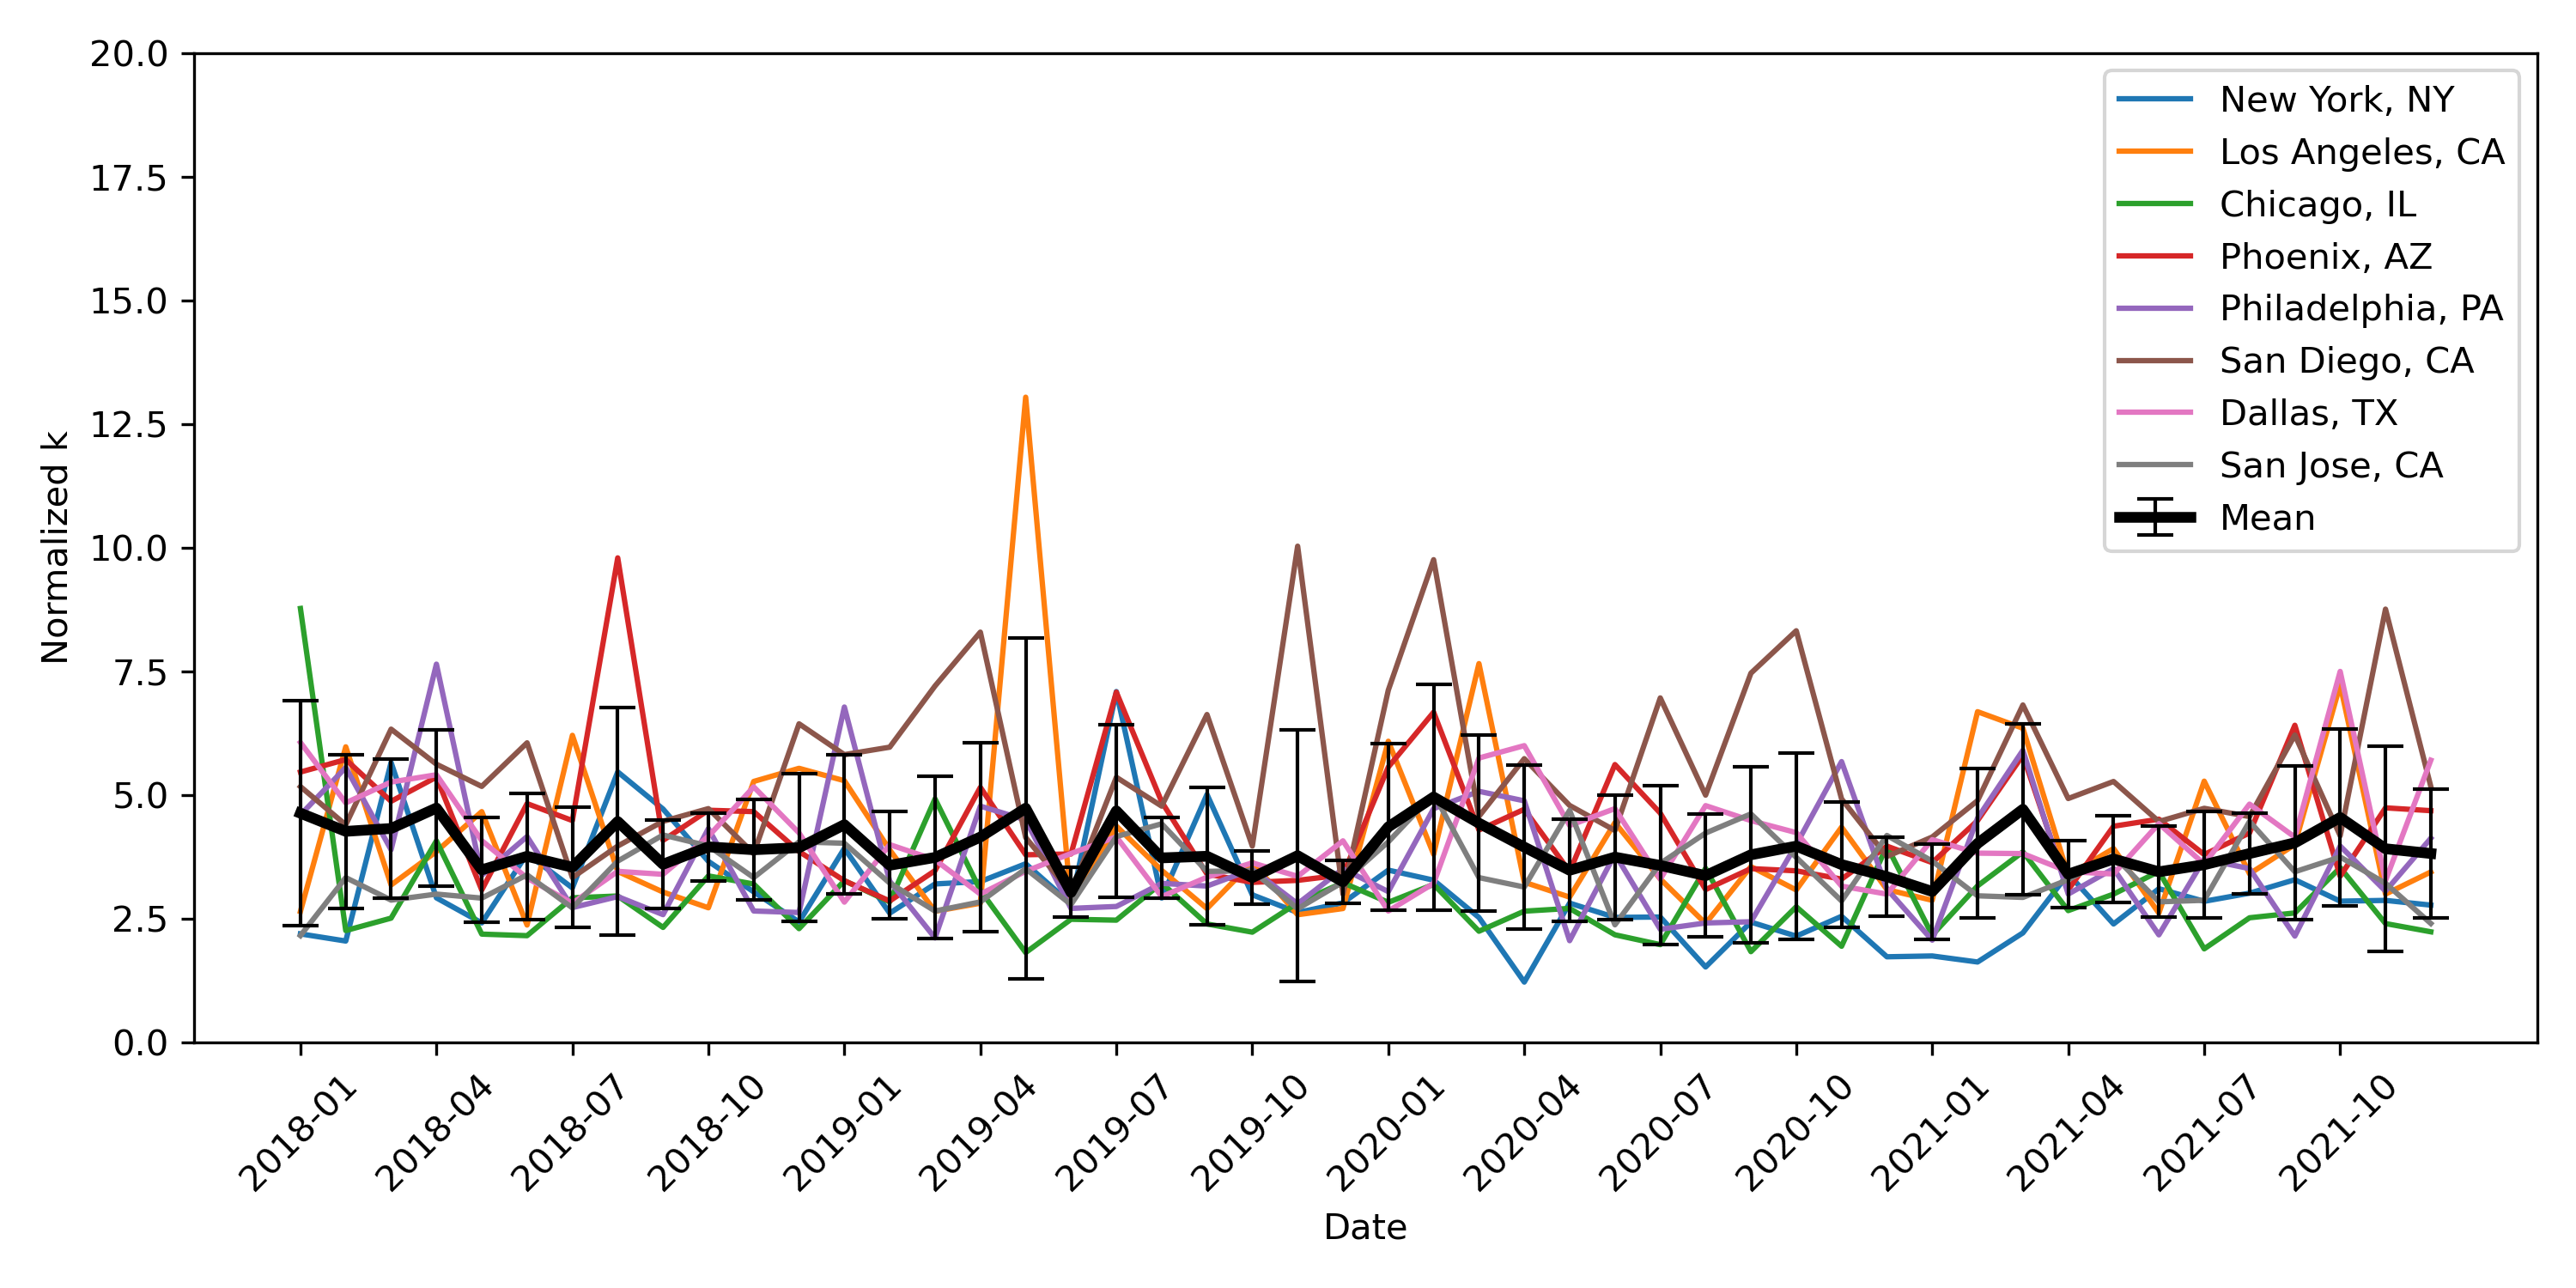}
        \caption{Normalized percolation thresholds based on the effective number of destinations (END) for each city over a 48-month period.}
        \label{fig: Normalized_k_across_time}
    \end{subfigure}
    \caption{Depiction of the variation in percolation thresholds over time. (a) shows the raw thresholds, and (b) shows the normalized thresholds based on the effective number of destinations (END). }
    \label{fig: overall_k_across_time}
\end{figure}

\begin{figure}
    \centering
    \includegraphics[width = \linewidth]{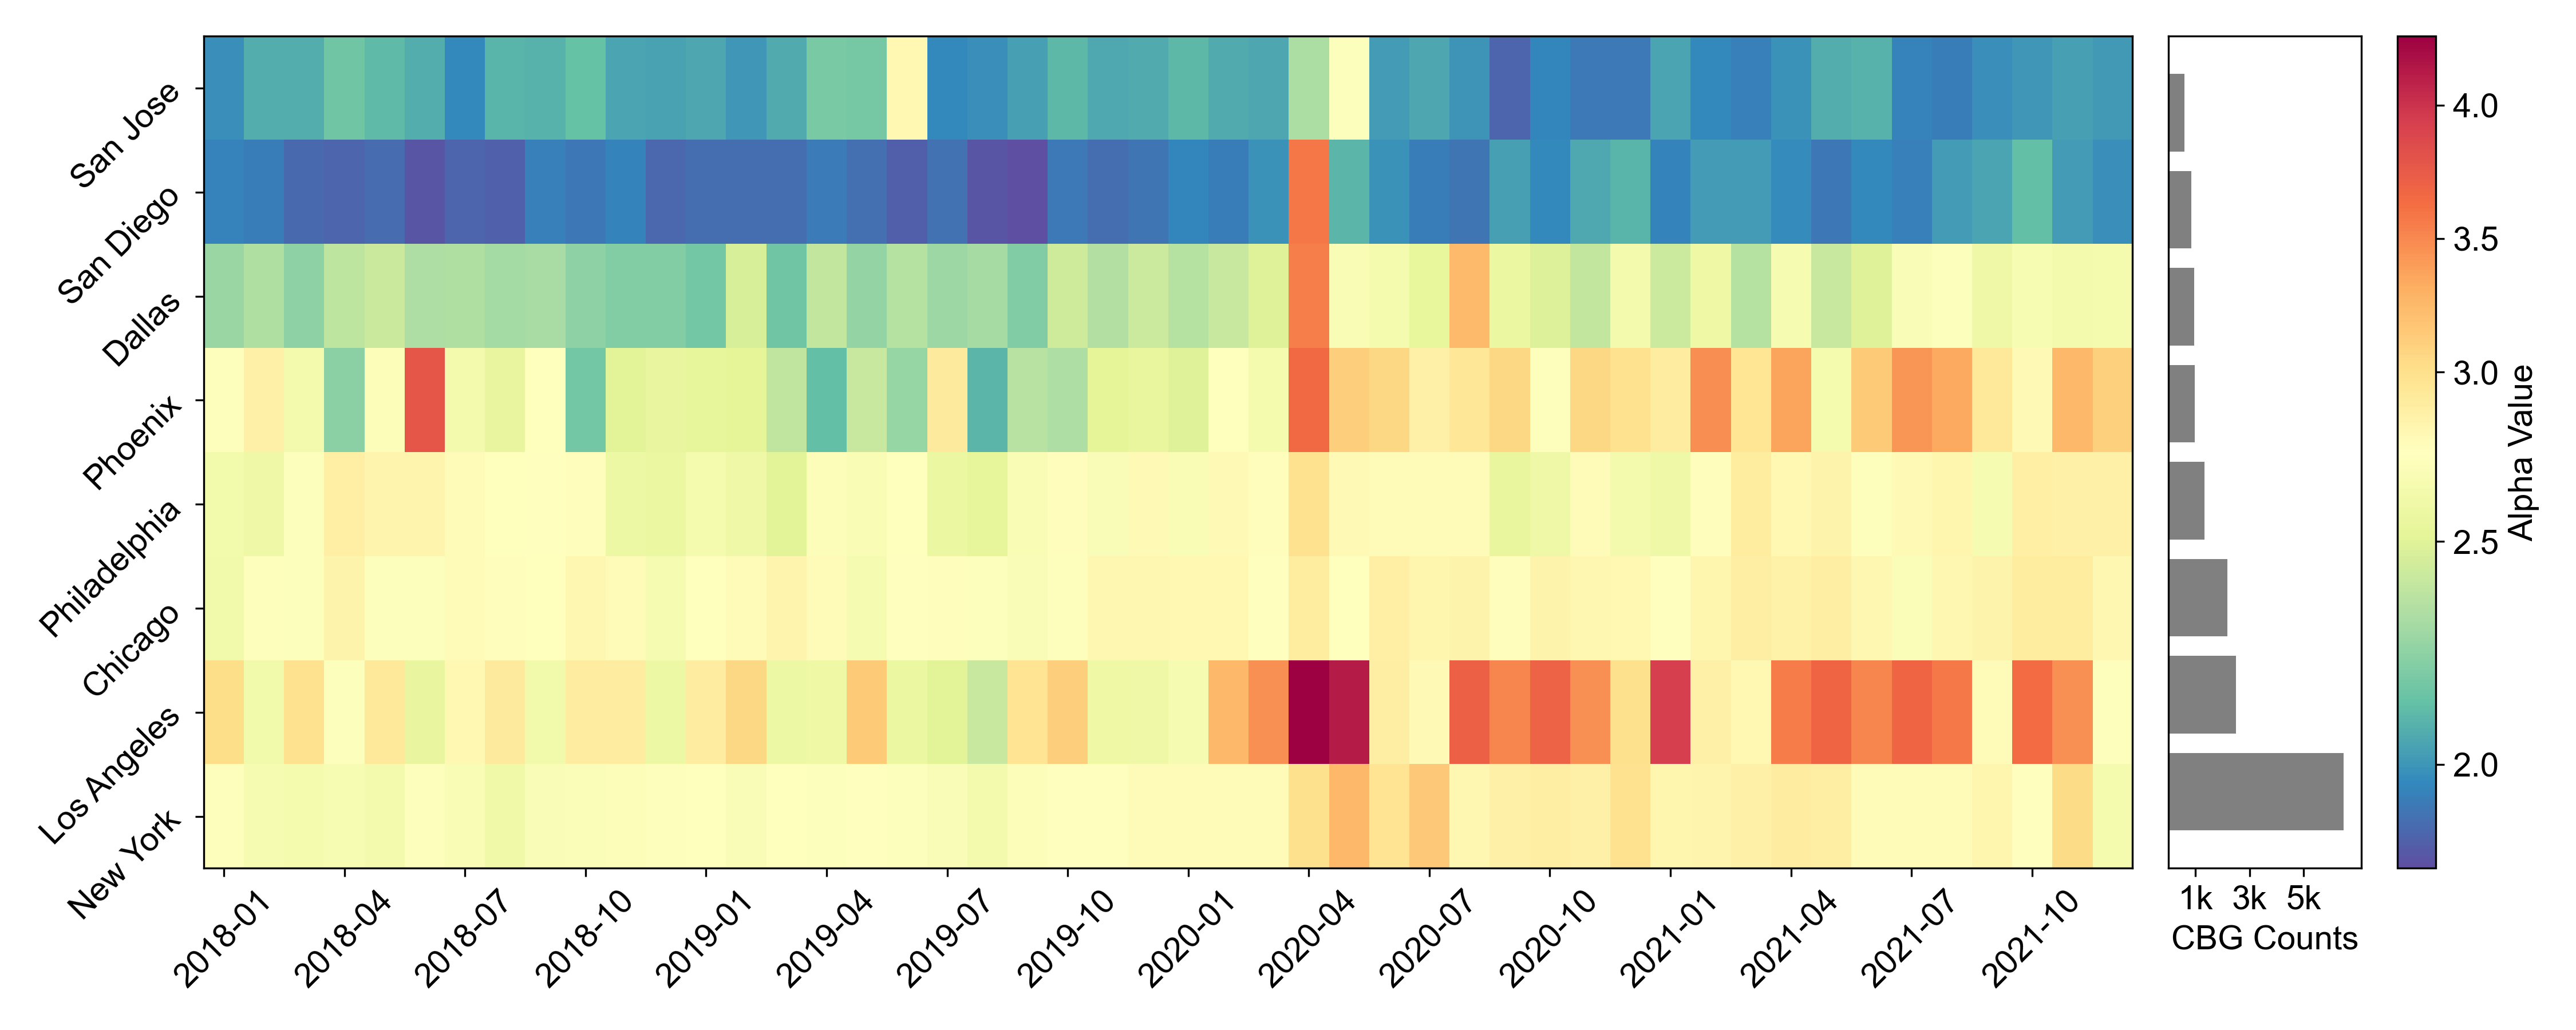}
    \caption{Comprehensive depiction of power-law exponents across different cities and time periods reveals two discernible trends. Longitudinally, there is a clear positive correlation between city size and alpha values. Laterally, a noticeable surge in alpha values is evident in the post-pandemic period. }
    \label{fig:powerlaw_exponents}
\end{figure}

\begin{figure}
    \centering
    \includegraphics[width = 0.6\linewidth]{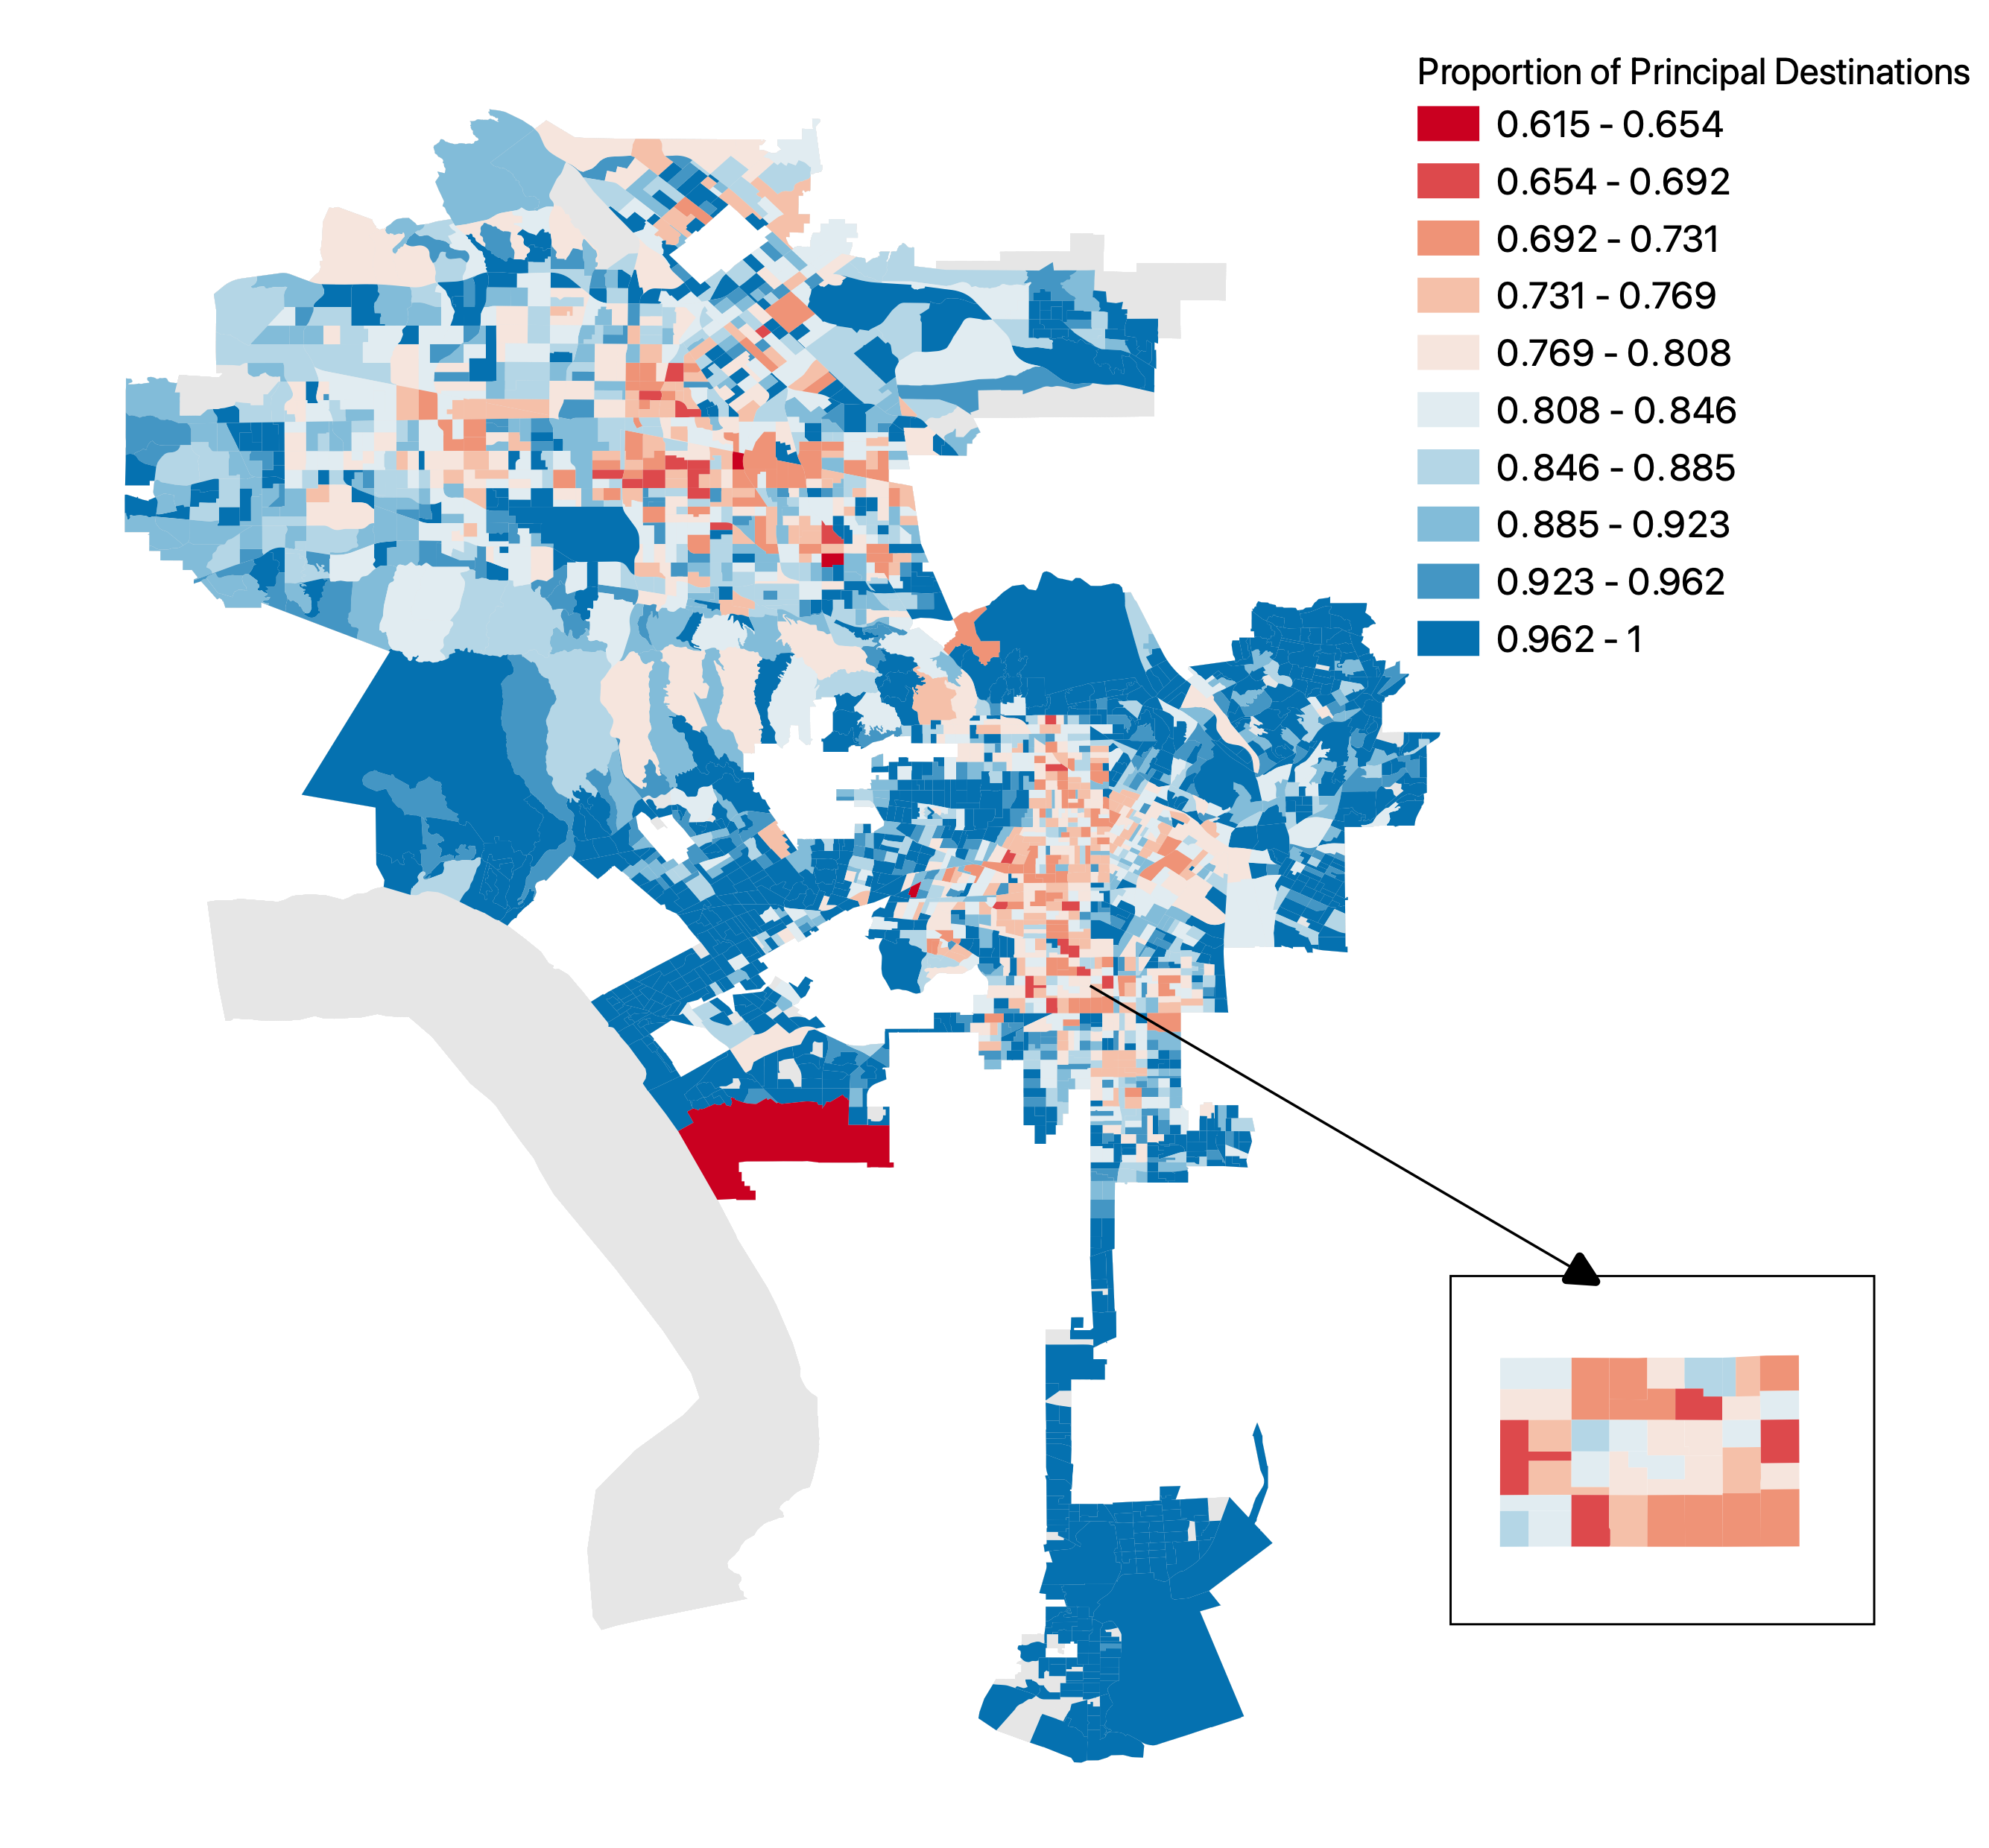}
    \caption{Spatial Distribution of the Proportion of Principal Destinations (PPD) in Los Angeles.  The inset provides a detailed view of Vermont Square, a neighborhood within the South Los Angeles region.}
    \label{fig:la_ppd}
\end{figure}

\begin{figure}
    \centering
    \includegraphics[width = 0.6\linewidth]{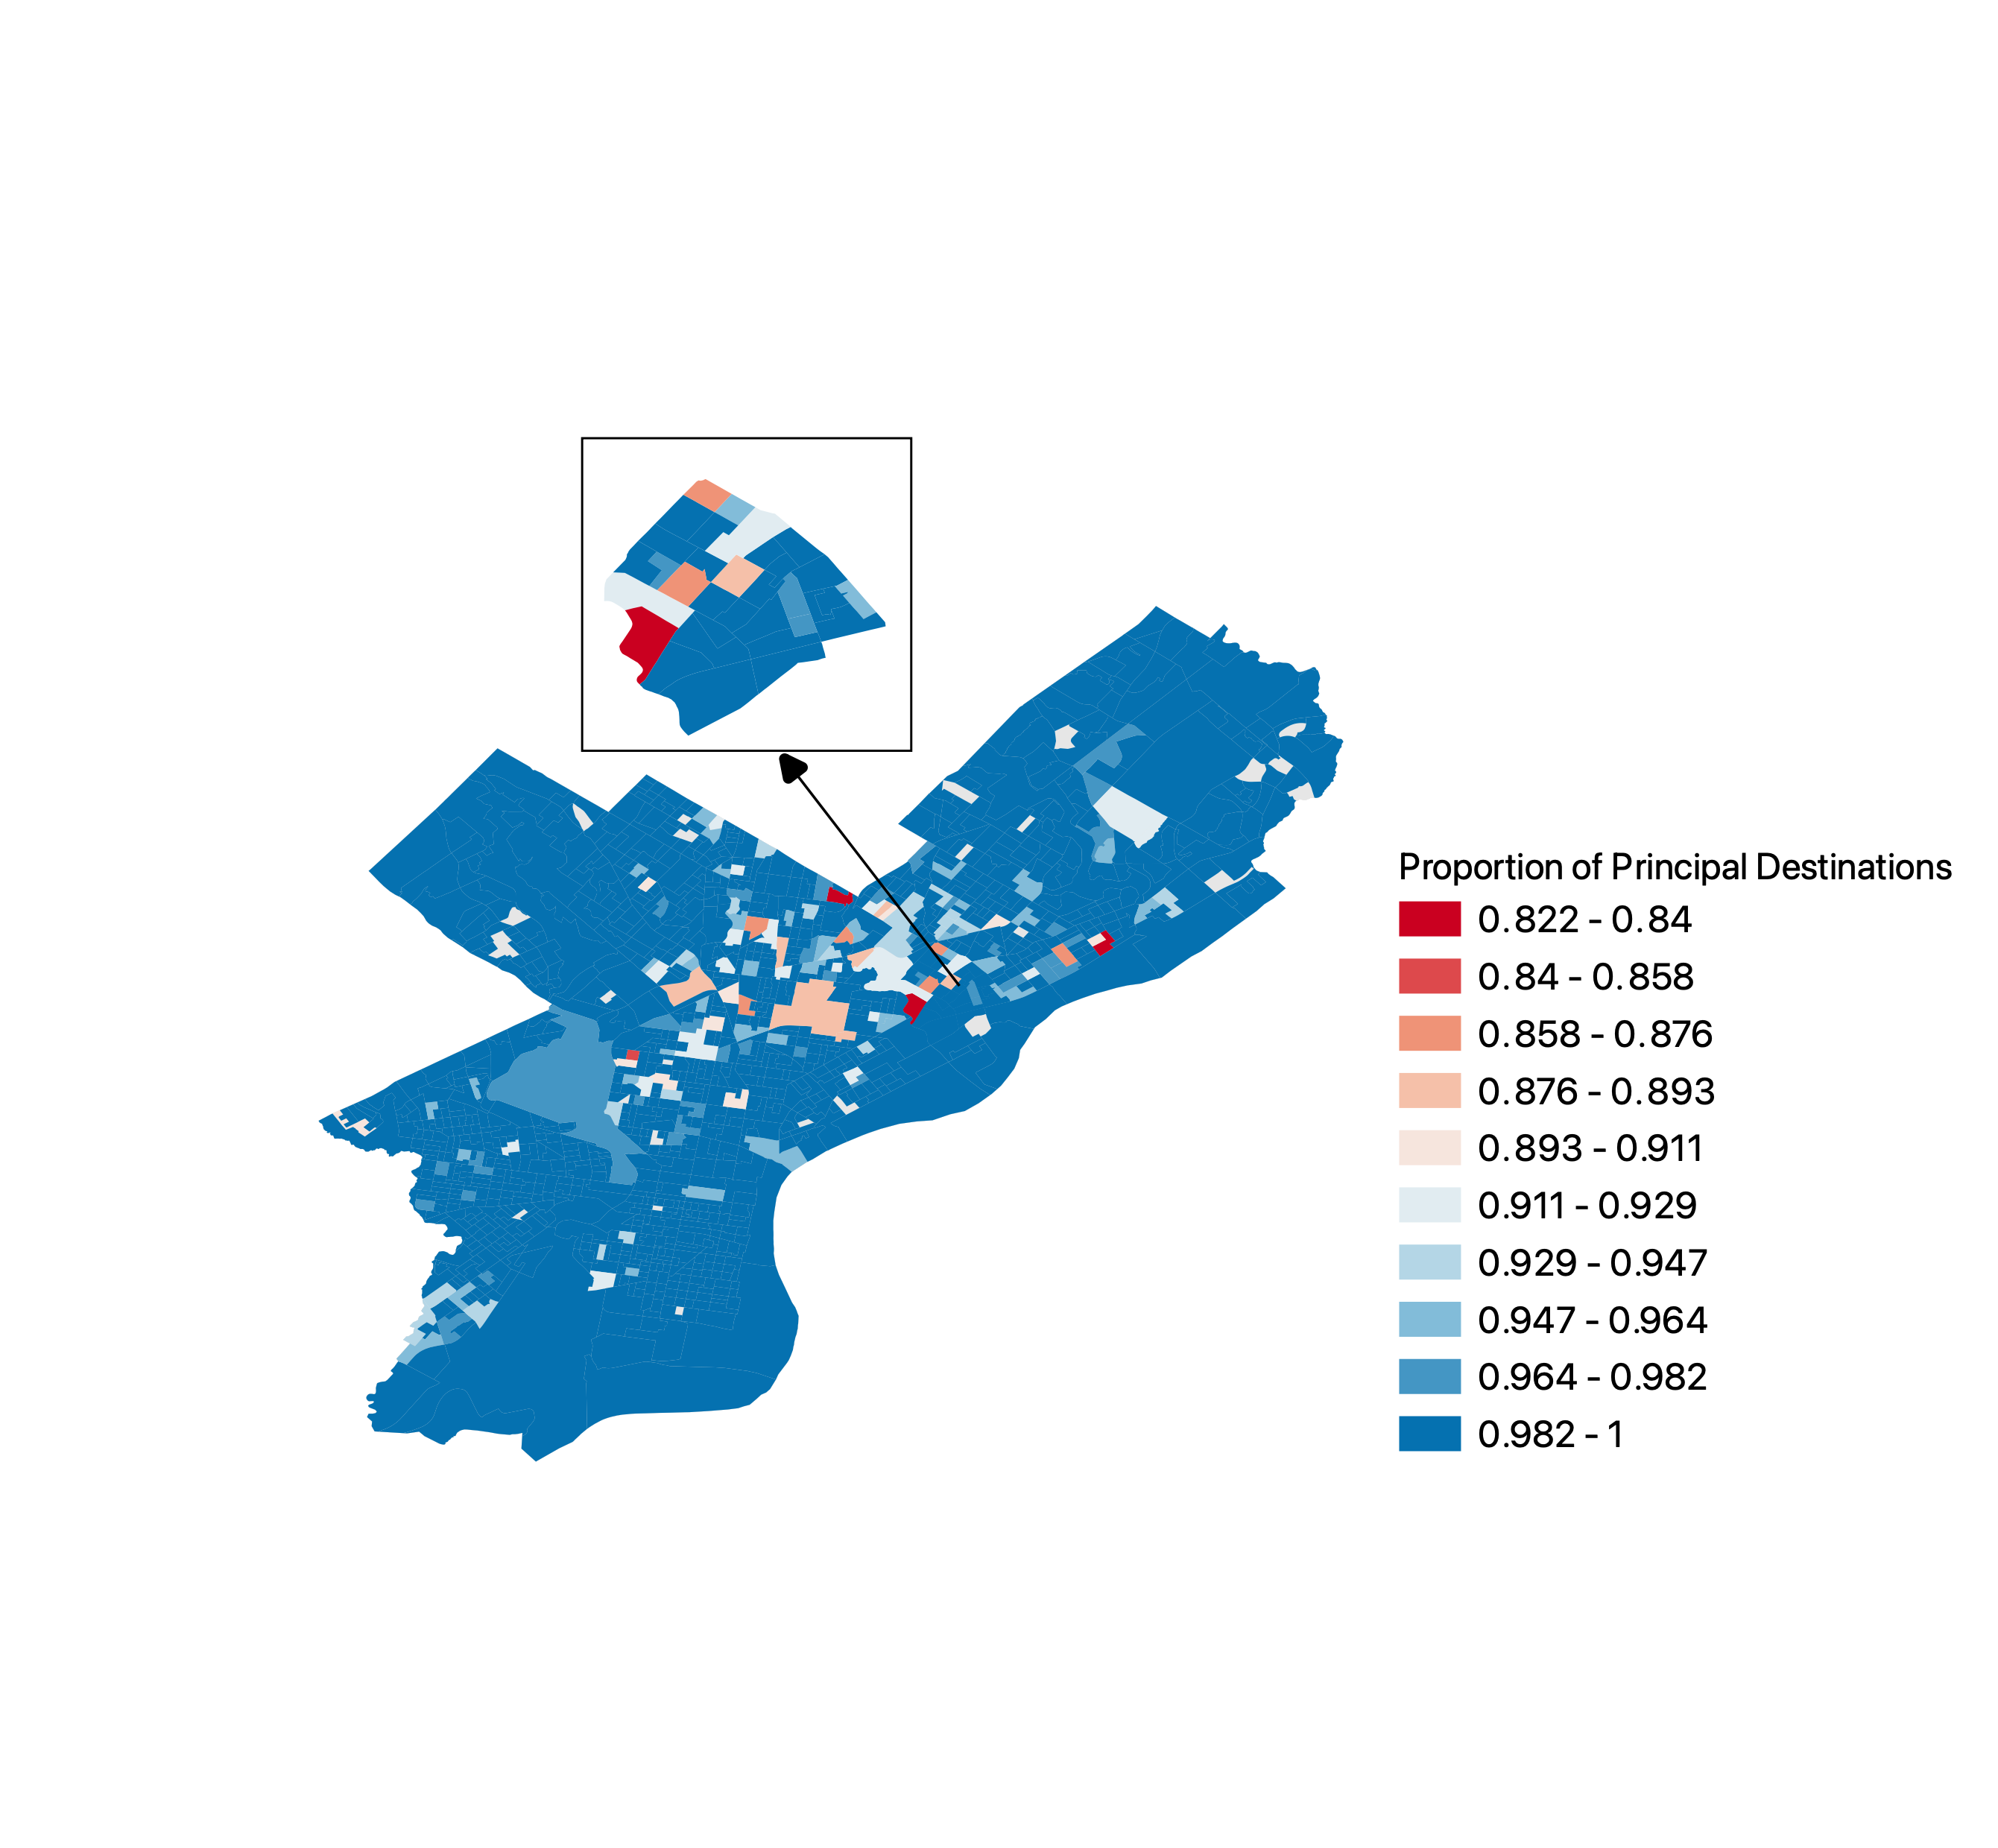}
    \caption{Spatial Distribution of the Proportion of Principal Destinations (PPD) in Philadelphia. The inset provides a detailed view of Frankford, a neighborhood in the Northeast section of Philadelphia.}
    \label{fig:philadelphia_ppd}
\end{figure}

\begin{figure}
    \centering
    \includegraphics[width=0.9\linewidth]{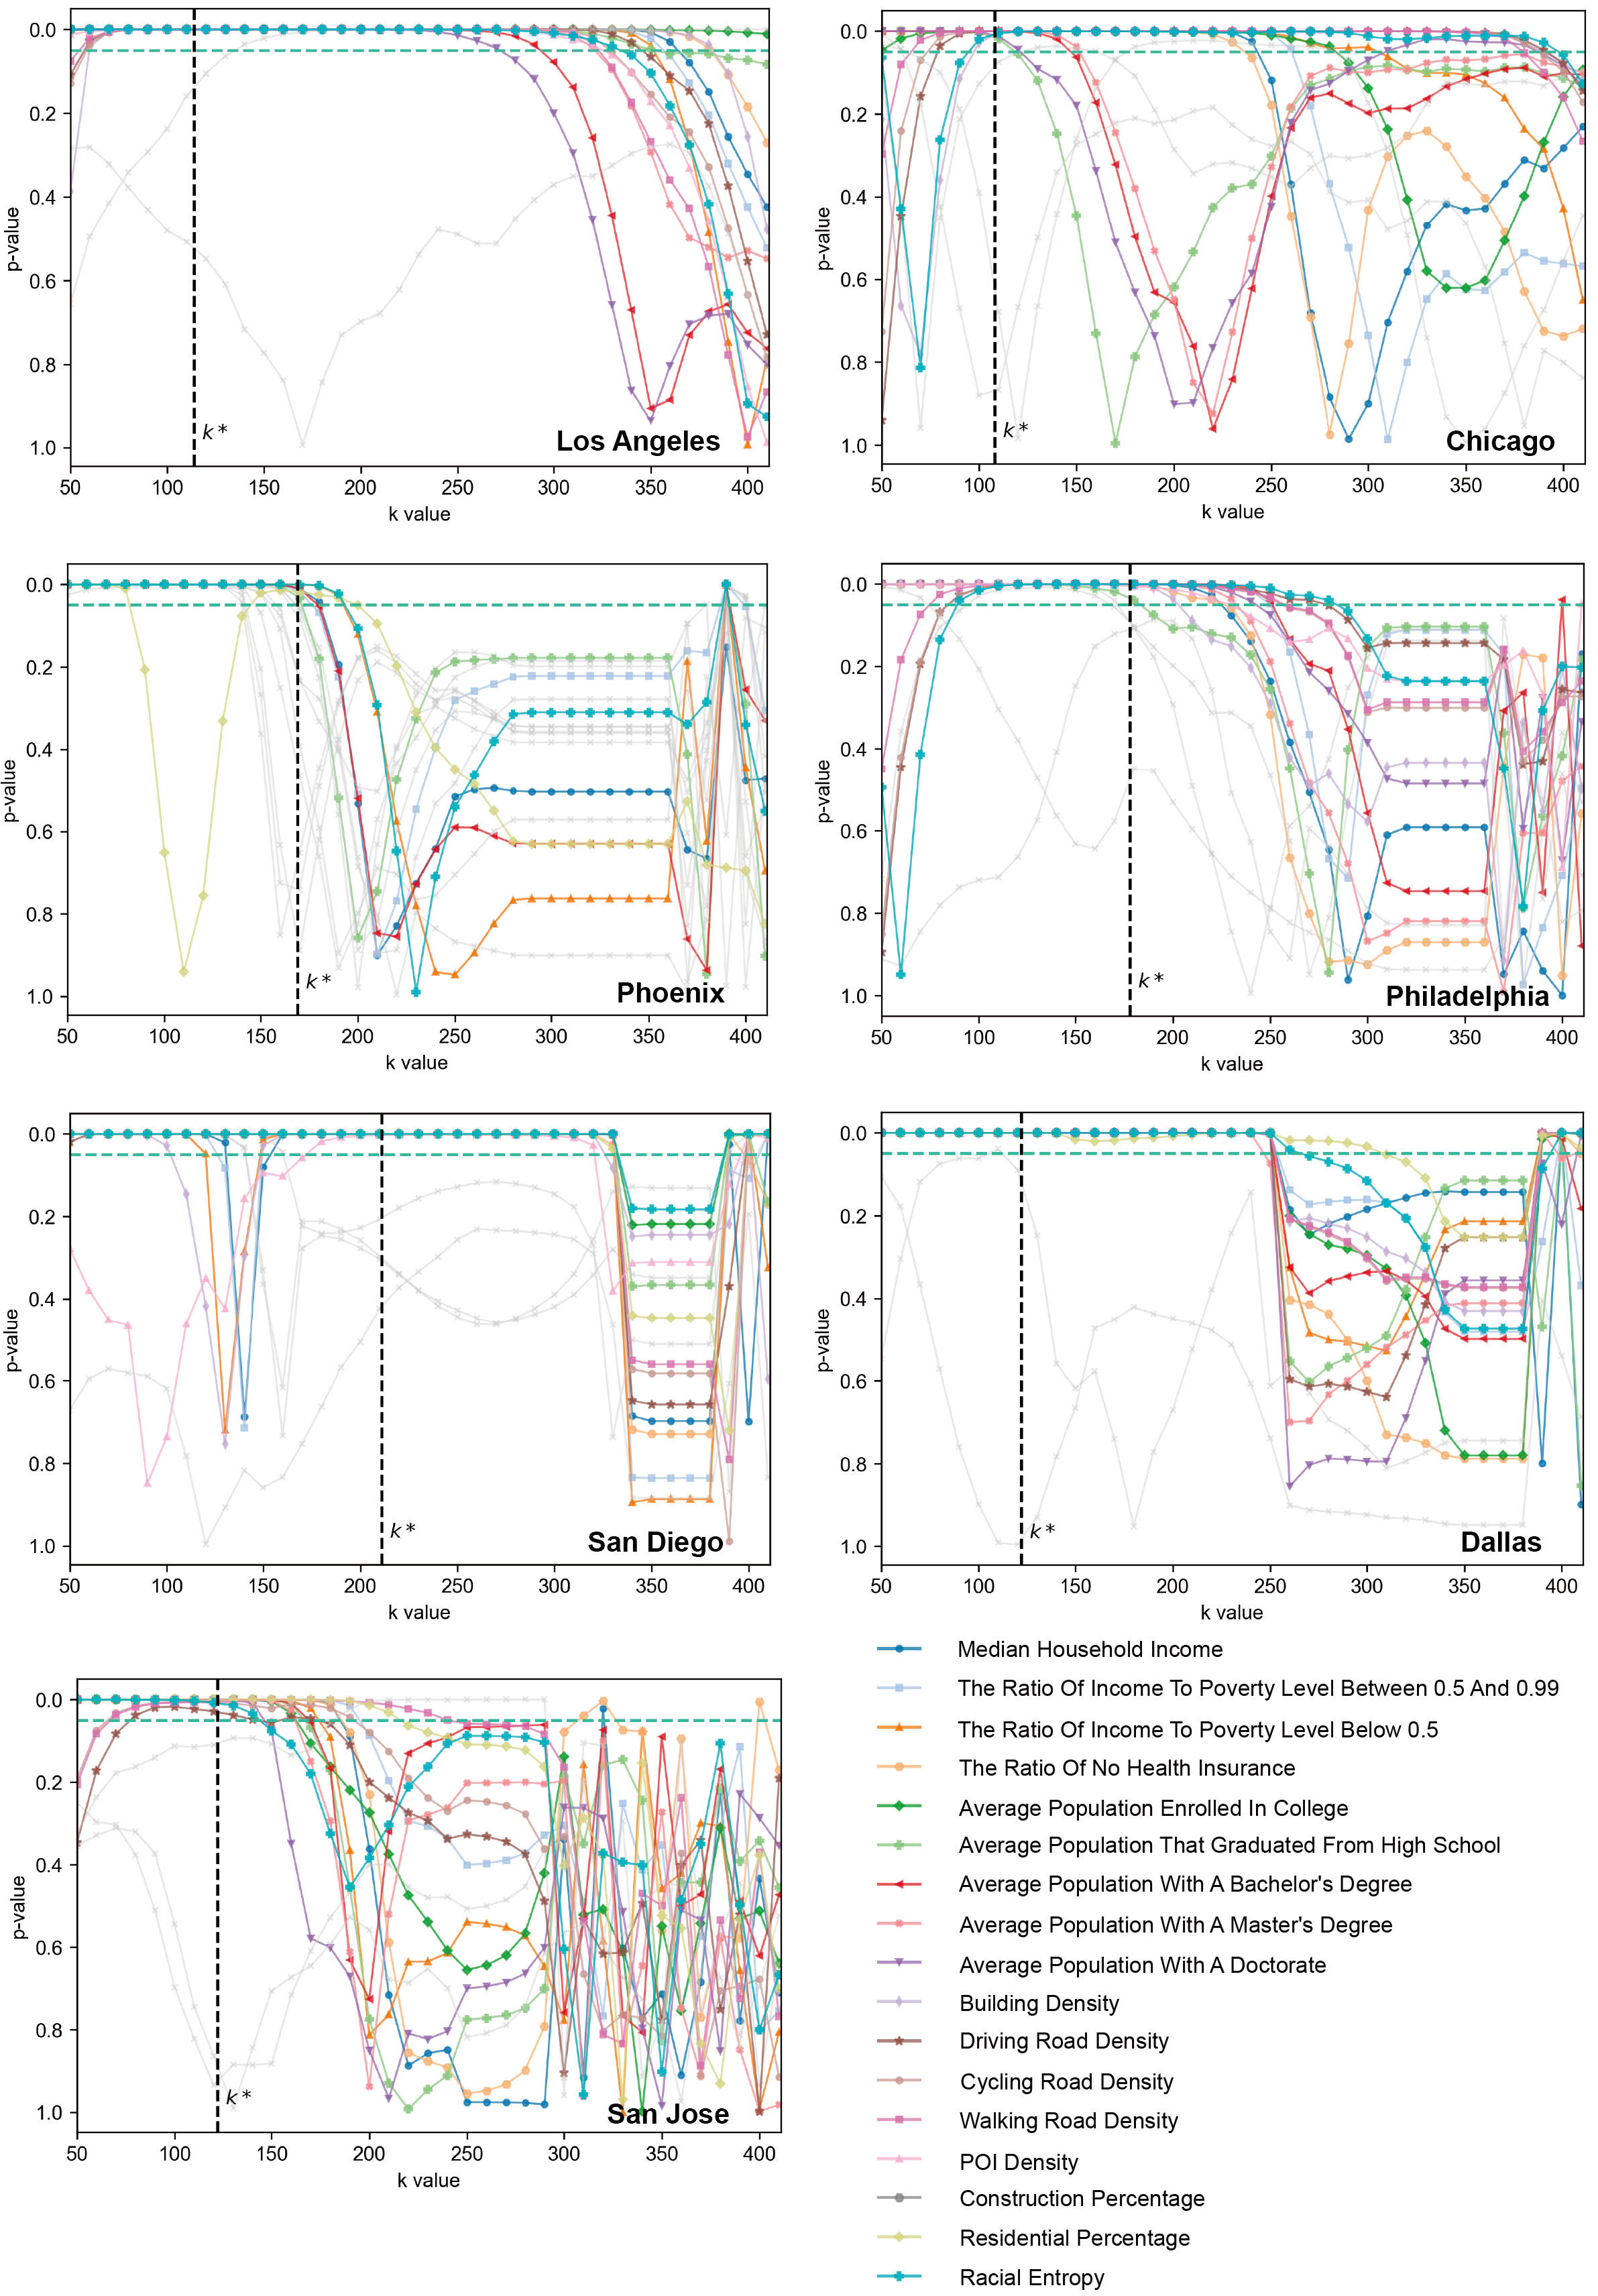}
    \caption{The relationship between the number of principal destinations and the $p$-value of regressions that link socioeconomic factors with the Proportion of Principal Destinations (PPD). Vertical black dashed lines represents the percolation threshold ($k^*$), and green horizontal dashed lines indicates a significance level of 0.05. Socioeconomic factors that show an insignificant correlation with PPD ($p$-value $>$ 0.05) at the percolation threshold are depicted in gray. Shifts in significance at $k^*$ are emphasized.}
    \label{fig:significance}
\end{figure}

\cleardoublepage

\input{supplementary.bbl}

\end{document}
